# Supplementary material for: Swarm Intelligence for Chemical Reaction Optimisation
Source: arXiv:2509.11798 source file (2025-09-15)
Supplement: Supplementary file 1 [file PSO_SI.pdf]

# Supplementary Information

## Swarm Intelligence for Chemical Reaction Optimisation

Rémi Schlama<sup>1,2†</sup>, Joshua W. Sin<sup>1,2\*†</sup>, Ryan P. Burwood<sup>3</sup>, Kurt Püntener<sup>1</sup>, Raphael Bigler<sup>1</sup>, Philippe Schwaller<sup>2,4\*</sup>

<sup>1</sup>Process Chemistry & Catalysis, Synthetic Molecules Technical Development,  
F. Hoffmann-La Roche AG, Basel, Switzerland

<sup>2</sup>Laboratory of Artificial Chemical Intelligence (LIAC), EPFL, Lausanne, Switzerland

<sup>3</sup>Solid State Sciences, Synthetic Molecules Technical Development,  
F. Hoffmann-La Roche AG, Basel, Switzerland

<sup>4</sup>National Centre of Competence in Research (NCCR) Catalysis, EPFL, Lausanne,  
Switzerland

†These authors contributed equally to this work.

\*Corresponding authors. Email: [wing-pong.sin@roche.com](mailto:wing-pong.sin@roche.com); [philippe.schwaller@epfl.ch](mailto:philippe.schwaller@epfl.ch)

## Contents

|          |                                                                      |           |
|----------|----------------------------------------------------------------------|-----------|
| <b>1</b> | <b>Parallel multi-objective chemical reaction optimisation</b>       | <b>3</b>  |
| 1.1      | Terminology and definitions for optimisation problems                | 3         |
| 1.2      | Chemical reaction optimisation                                       | 3         |
| 1.3      | Featurising reaction conditions                                      | 4         |
| 1.4      | Bayesian optimisation                                                | 4         |
| <b>2</b> | <b>Particle swarm optimisation (PSO)</b>                             | <b>5</b>  |
| 2.1      | Swarm communication topologies for batched PSO                       | 5         |
| 2.2      | Canonical PSO                                                        | 6         |
| 2.3      | $\alpha$ -PSO: Machine learning-augmented PSO                        | 8         |
| <b>3</b> | <b>Emulated benchmark datasets</b>                                   | <b>10</b> |
| 3.1      | Creating virtual benchmarks with experimental data                   | 10        |
| 3.2      | Analysing reaction landscape topology with local Lipschitz constants | 10        |
| <b>4</b> | <b>Computational benchmarks</b>                                      | <b>16</b> |
| 4.1      | Baseline benchmarks                                                  | 16        |
| 4.1.1    | Buchwald-Hartwig dataset                                             | 16        |
| 4.1.2    | Ni-Suzuki dataset                                                    | 17        |
| 4.2      | Effect of cognitive and social coefficients                          | 17        |
| 4.2.1    | Buchwald-Hartwig dataset                                             | 18        |
| 4.2.2    | Ni-Suzuki dataset                                                    | 25        |
| 4.3      | Effect of particle re-initialisation                                 | 31        |
| 4.3.1    | Buchwald-Hartwig dataset                                             | 32        |
| 4.3.2    | Ni-Suzuki dataset                                                    | 32        |

|          |                                                         |           |
|----------|---------------------------------------------------------|-----------|
| <b>5</b> | <b>Implementation details</b>                           | <b>33</b> |
| <b>6</b> | <b>High-throughput experimentation (HTE) platform</b>   | <b>34</b> |
| <b>7</b> | <b>Prospective application: Sulfonamide coupling</b>    | <b>35</b> |
| 7.1      | Chemical space description . . . . .                    | 35        |
| 7.2      | HTE experimental procedure . . . . .                    | 36        |
| 7.3      | Landscape topology analysis . . . . .                   | 36        |
| 7.4      | Statistical analysis . . . . .                          | 37        |
| <b>8</b> | <b>Prospective application: Suzuki-Miyaura reaction</b> | <b>39</b> |
| 8.1      | Chemical space description . . . . .                    | 39        |
| 8.2      | HTE experimental procedure . . . . .                    | 40        |
| 8.3      | Landscape topology analysis . . . . .                   | 40        |

# 1 Parallel multi-objective chemical reaction optimisation

## 1.1 Terminology and definitions for optimisation problems

In this section, we define the terminology and concepts used in this work. In an optimisation problem, we denote the search space  $\mathcal{X}$  as the space of all possible solutions. We seek to identify the solution that maximises the objective function  $f : \mathcal{X} \rightarrow \mathbb{R}$ . The optimisation problem can be formulated as finding  $\mathbf{x}^*$ , where

$$\mathbf{x}^* = \arg \max_{\mathbf{x} \in \mathcal{X}} f(\mathbf{x}). \quad (1)$$

When extended to multi-objective optimisation problems, we seek to optimise multiple objectives simultaneously. The objective function  $f : \mathcal{X} \rightarrow \mathbb{R}^m$  maps each solution  $\mathbf{x} \in \mathcal{X}$  to  $m$  objective values, yielding the vector  $\mathbf{f}(\mathbf{x}) = [f_1(\mathbf{x}), f_2(\mathbf{x}), \dots, f_m(\mathbf{x})]^\top$ . Since the  $m$  objectives often conflict, there is typically no single solution that simultaneously optimises all objectives. Instead, our goal is to identify Pareto optimal solutions, the set of all non-dominated solutions [1–3]. A solution  $\mathbf{x}$  dominates another solution  $\tilde{\mathbf{x}}$  if  $f_i(\mathbf{x}) \geq f_i(\tilde{\mathbf{x}})$  for all  $i \in \{1, 2, \dots, m\}$  and  $f_i(\mathbf{x}) > f_i(\tilde{\mathbf{x}})$  for at least one  $i \in \{1, 2, \dots, m\}$ . Correspondingly, a solution is non-dominated if no other solution achieves better or equal performance in all objectives while being strictly better in at least one objective. Optimisation towards the Pareto front can be achieved through different approaches, such as converting the optimisation problem into a single-objective optimisation by maximising a scalar combination of the objectives,  $s : \mathbb{R}^m \rightarrow \mathbb{R}$ , or by optimising the hypervolume indicator [1].

The hypervolume indicator provides a quantitative measure for evaluating the quality of a set of multi-objective solutions. Given a set of solutions and a fixed reference point in objective space, the hypervolume calculates the volume of objective space dominated by these solutions. For a set of solutions  $S = \{\mathbf{x}_1, \mathbf{x}_2, \dots, \mathbf{x}_k\}$  and a reference point  $r \in \mathbb{R}^m$ , the hypervolume  $HV(S)$  quantifies the  $m$ -dimensional volume bounded by the objective vectors in  $\mathbf{f}(S) = \{\mathbf{f}(\mathbf{x}_1), \mathbf{f}(\mathbf{x}_2), \dots, \mathbf{f}(\mathbf{x}_k)\}$  and the reference point  $r$ . The hypervolume indicator captures both convergence towards optimal objectives and diversity of solutions across the objective space. A larger hypervolume indicates better overall performance, reflecting the identification of solutions that are both high-performing and well-distributed across different trade-offs between objectives. In this work, we use the hypervolume indicator to compare the effectiveness of different multi-objective optimisation algorithms.

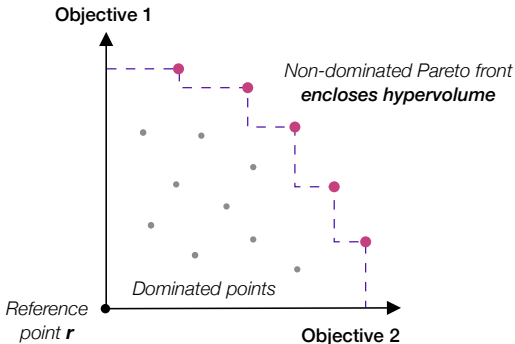

## 1.2 Chemical reaction optimisation

In a reaction optimisation campaign, we aim to find reaction conditions that maximise single or multiple reaction outcomes. Reaction conditions are typically described using both categorical variables (e.g., catalysts, ligands, bases) and continuous variables (e.g., temperature, concentration). We discretise continuous variables by selecting representative values within their ranges, as minor variations within these ranges often have a negligible impact on reaction outcomes. The reaction condition search space  $\mathcal{X}$  is the Cartesian product of the sets of feasible options for each of the  $N$  reaction variables  $\mathcal{X} = \mathcal{V}_1 \times \mathcal{V}_2 \times \dots \times \mathcal{V}_N$ . Here, each  $\mathcal{V}_i$  is a set of feasible options for a specific reaction component (e.g., solvents). The goal of the reaction optimisation campaign is to identify reaction conditions within  $\mathcal{X}$  that optimise the reaction outcome objective function  $f : \mathcal{X} \rightarrow \mathbb{R}^m$ .

### 1.3 Featurising reaction conditions

In the reaction optimisation campaigns explored in this study, a large number of categorical reaction variables such as ligands, solvents, co-solvents, and precatalysts were considered, each of which needs to be appropriately represented numerically to enable effective modelling. While one-hot encoding (OHE) could be employed, many OHE vectors would be required when the number of categories is large. For instance, we explored up to 82 different ligands in some campaigns. To provide more chemically meaningful and compact representations, we instead featurised ligands and solvents using quantum mechanical descriptors, which have demonstrated strong performance in many prior reaction optimisation studies [4–7]. For monophosphine ligands, we used 190 density functional theory (DFT) descriptors obtained from the Kraken featurisation workflow [8]. Given the high dimensionality of this descriptor set and the limited number of data points available for training machine learning (ML) surrogate models, we applied Principal Component Analysis (PCA) for dimensionality reduction. PCA components explaining 99% of the variance were retained, thereby capturing essential chemical variation while maintaining a condensed input space. Solvent descriptors from Moity et al. [9] were used and parameterised using COSMOtherm, represented by four DFT-based features and labelled Solvent *F1* to Solvent *F4*. The remaining categorical variables in our study (co-solvents, bases, and precatalysts) were represented using one-hot encoding. The temperature variable was retained as a discretised numerical feature.

### 1.4 Bayesian optimisation

Bayesian optimisation (BO) is a popular algorithmic approach for the optimisation of black-box functions, particularly in settings where experiments are expensive and time-consuming [10]. Recent advances in ML have led to the widespread adoption of BO in the chemical sciences, with numerous experimental case studies demonstrating its ability to outperform traditional strategies such as one-variable-at-a-time (OVAT) and purely expert-guided design [5, 11, 12]. BO has proven especially valuable in chemical reaction optimisation, where complex reactivity landscapes, limited experimental budgets, and high-dimensional input spaces are common challenges. At its core, BO is a sequential model-based optimisation framework. BO operates by constructing a probabilistic surrogate model, typically a Gaussian Process (GP), to approximate the unknown objective function [10]. This GP surrogate models both the predicted outcomes and their associated uncertainties, which are used by an acquisition function to propose the next set of experiments to evaluate. The acquisition function balances exploration, by sampling uncertain regions of the design space, and exploitation, by focusing on areas with high predicted performance, driving data-efficient search strategies in low-data regimes. However, BO’s reliance on complex probabilistic models makes it challenging for practitioners to understand model logic and optimisation behaviour, motivating the development of more interpretable optimisation approaches. The emergence of robotic high-throughput experimentation (HTE) platforms has further amplified the utility of BO. HTE platforms facilitate miniaturised and parallelised exploration of reaction conditions, reducing cycle times and enabling broader search across chemical space [13, 14]. When integrated with BO, this allows for highly-parallel and data-efficient optimisation [5]. In this work, we employed BO using the Minerva platform as a baseline benchmark strategy against  $\alpha$ -PSO. Specifically, we used the q-Noisy Expected Hypervolume Improvement (qNEHVI) [3] acquisition function, which has demonstrated superior empirical performance in batch reaction optimisation over other acquisition functions across multiple computational and experimental studies. In our overall BO workflow, initial reaction conditions were selected with Sobol sampling [15] to ensure broad coverage of the search space and increase the likelihood of identifying informative regions. A GP regression model was then trained on the collected data to model reaction outcomes (e.g., yield, selectivity), and predictions were used to compute the acquisition function. For additional technical background and a formal mathematical treatment of BO, the reader is referred to Frazier [10].

## 2 Particle swarm optimisation (PSO)

### 2.1 Swarm communication topologies for batched PSO

We describe here methods for formalising the communication topology of particles in Particle Swarm Optimisation (PSO) [16]. The communication topology defines how information is shared between particles within the swarm. Canonical PSO employs two primary communication topologies: Lbest (local best) and Gbest (global best) [17–19]. In the Lbest topology, each particle communicates with only its  $k$  immediate neighbours (usually  $k = 2$ ), creating a ring network structure where information propagates gradually through the swarm (Supplementary Figure 1). Conversely, the Gbest topology comprises a complete graph  $K_{n_p}$ , where  $n_p$  represents the number of particles in the swarm (e.g., in Supplementary Figure 1,  $n_p = 10$ ). This complete connectivity means that whenever any particle discovers a new global optimum, this information is available to all other particles in the swarm, directing their subsequent movements. While both topologies provide distinct advantages, we adopted Gbest for  $\alpha$ -PSO as the fully connected information flow facilitates efficient communication across our large, parallel experimental batches of up to 96 reactions. Both topologies can be implemented with either synchronous or asynchronous particle updates. In asynchronous PSO, particles are processed sequentially, with each particle being evaluated (e.g., obtaining its yield) and immediately updated before proceeding to the next particle, similar to single-batch reaction optimisation. This allows newly discovered results to immediately influence the processing of subsequent particles. However, parallel batched experimental settings require synchronous updates since experimental results are only available after completing an entire batch of experiments. We therefore employ Synchronous PSO (SPSO) [20] in  $\alpha$ -PSO, where all particles in a batch are evaluated first, then all particles are updated simultaneously using the same information from the completed experiments (Supplementary Figure 1).

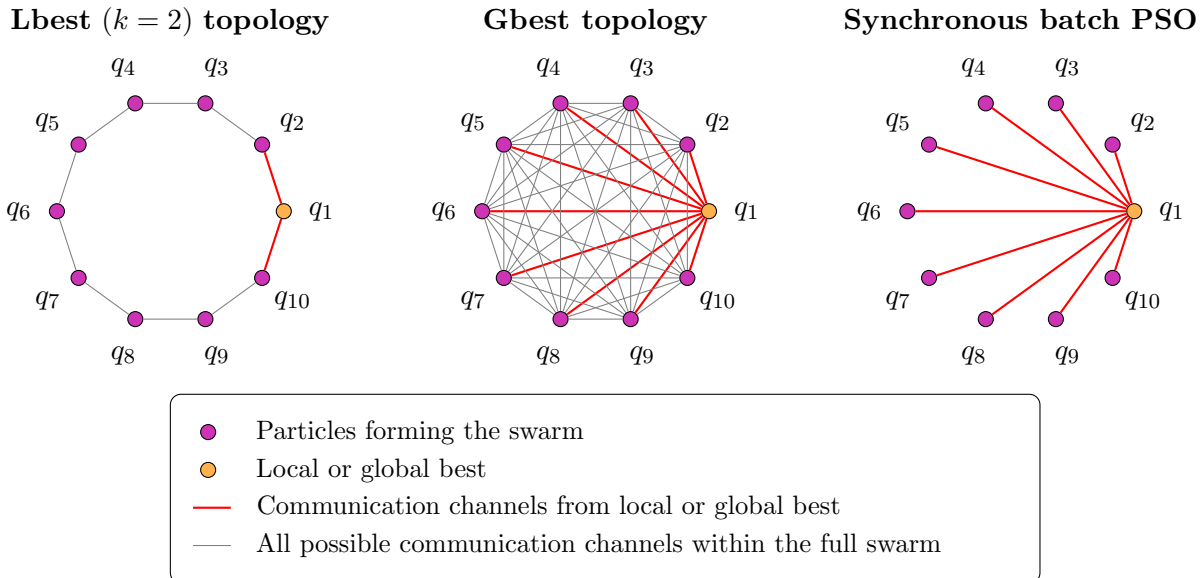

**Supplementary Figure 1: Comparison of communication topologies for the PSO algorithm.** **Left:** Lbest topology ( $k = 2$ ), each particle can communicate with its two closest neighbours, creating a ring network where information propagates gradually through the swarm. **Middle:** Gbest topology, showing the complete connectivity network where each particle can communicate with all other particles in the swarm. **Right:** Information flow in Gbest topology during synchronous batch evaluation, where all particles simultaneously receive information from the global best particle.

## 2.2 Canonical PSO

PSO is a population-based meta-heuristic optimisation algorithm inspired by the collective behaviour of bird flocks and fish schools foraging in nature [16]. PSO explores a search space  $\mathcal{X}$  using a swarm of particles, each possessing a position and velocity that evolves over each optimisation iteration. Particles communicate through a defined network topology (see Section 2.1) and are guided by two sources of information: the global best position discovered by any particle in the swarm, and each particle’s personal best position from their own search history. Formally, each particle  $j$  is defined as a triplet  $q_j = (\mathbf{x}_j, \mathbf{v}_j, \mathbf{p}_j)$ , where  $\mathbf{x}_j \in \mathcal{X}$  denotes the current position,  $\mathbf{v}_j \in \mathbb{R}^d$  represents the velocity vector, and  $\mathbf{p}_j \in \mathcal{X}$  stores the personal best position that yielded the highest objective value so far for that particle. A swarm comprising  $n_p$  particles is defined as the set  $\mathcal{S} = \{q_j\}_{j=1}^{n_p}$ . PSO proceeds iteratively by updating each particle’s velocity and position. The velocity update incorporates two behavioural components: a cognitive term weighted by coefficient  $c_1$  that directs the particle toward its personal best position, and a social term weighted by coefficient  $c_2$  that guides the particle toward the global best position  $\mathbf{g}$  discovered so far by the swarm. The velocity and position update equations are:

$$\mathbf{v}_j^{(i+1)} = \omega \mathbf{v}_j^{(i)} + \left( \mathbf{p}_j^{(i)} - \mathbf{x}_j^{(i)} \right) \odot \phi_1 + \left( \mathbf{g}^{(i)} - \mathbf{x}_j^{(i)} \right) \odot \phi_2 \quad (2)$$

$$\mathbf{x}_j^{(i+1)} = \mathbf{x}_j^{(i)} + \mathbf{v}_j^{(i+1)} \quad (3)$$

Where  $\phi_1 = c_1 \mathbf{r}_1$ ,  $\phi_2 = c_2 \mathbf{r}_2$ ,  $\mathbf{r}_1, \mathbf{r}_2 \sim \mathcal{U}(\mathbf{0}, \mathbf{1})$  are random vectors drawn from a uniform distribution.  $c_1, c_2 \in \mathbb{R}$  are respectively the cognitive coefficient and social coefficient.  $\omega \in \mathbb{R}$  is the inertia weight and  $\odot$  denotes the Hadamard product. The superscript  $(i)$  indicates the iteration number.

PSO can be adapted for chemical reaction optimisation by representing each reaction condition as a particle position in the combinatorial space of all possible reaction condition combinations. At each iteration, particles move to new positions, corresponding to new reaction conditions to evaluate experimentally. Each particle requires an objective score to guide the swarm toward optimal solutions, defining the objective space that particles navigate during optimisation. This score can represent any experimental outcome requiring optimisation, such as reaction yield, selectivity, or cost. For multi-objective optimisation scenarios (e.g., maximising both yield and selectivity), we use a scalarisation function  $\mathbf{s}$  that combines the multiple objectives into a single scalar score. In the context of batched high-throughput experimentation (HTE), each reaction in a HTE plate corresponds to a particle position in a normalised reaction condition search space  $\mathcal{X}$ . The experimental results from the HTE plate define the objective values used to guide particle movement in PSO iterations. We outline our implementation of canonical PSO adapted for parallel reaction optimisation in Algorithm 1.

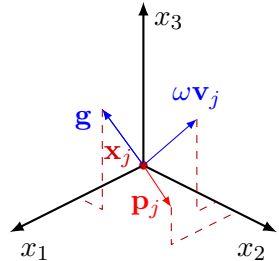

---

**Algorithm 1:** Canonical Particle Swarm Optimisation Algorithm (batch evaluation)

---

**Input** :  $\mathcal{X}$ , a normalised feature search space,  $\mathbf{f} : \mathcal{X} \rightarrow \mathbb{R}^m$ , an objective function with  $m$  objectives,  $\left\{q_j = \left(\mathbf{x}_j^{(i)}, \mathbf{v}_j^{(i)}, \mathbf{p}_j^{(i)}\right)\right\}_{j=1}^{n_p}$ , a set of  $n_p$  particles,  $c_1 \in \mathbb{R}$ , a cognitive parameter,  $c_2 \in \mathbb{R}$ , a social parameter,  $\omega \in \mathbb{R}$ , an inertia weight,  $n_i$ , the number of iterations,  $n_p$ , the number of particles forming the swarm,  $\mathbf{s} : \mathbb{R}^m \rightarrow \mathbb{R}$ , a scalarisation function combining multiple objectives into a single score,  $d \in \mathbb{N}$ , the dimensionality of the search space.

**Output:** An approximate global best position  $\mathbf{g}$  that maximises  $\mathbf{f}$ .

```
/* Initialisation of the particles */
for  $j \leftarrow 1$  to  $n_p$  do
     $\mathbf{x}_j^{(0)} \leftarrow \arg \min_{\mathbf{x}_k \in \mathcal{X}} \left( \|\mathbf{x}_j^0 - \mathbf{x}_k\|_2 \right)$ ,  $\mathbf{x}_j^0 \sim \mathcal{LDS}(d, j)$ ;
     $\mathbf{p}_j^{(0)} \leftarrow \mathbf{x}_j^{(0)}$ ;
     $\mathbf{v}_j^{(0)} \leftarrow \mathbf{0}$ ;

/* Evaluate positions using objective function f */
 $j^* \leftarrow \arg \max_j s(\mathbf{f}(\mathbf{x}_j^{(0)}))$ ;
 $\mathbf{g}^{(0)} \leftarrow \mathbf{x}_{j^*}^{(0)}$ ;

/* Optimisation loop */
for  $i \leftarrow 0$  to  $n_i - 1$  do
    for  $j \leftarrow 1$  to  $n_p$  do
         $\phi_1 \leftarrow c_1 \cdot \mathbf{r}_1$ ,  $\mathbf{r}_1 \sim \mathcal{U}(\mathbf{0}, \mathbf{1})$ ;
         $\phi_2 \leftarrow c_2 \cdot \mathbf{r}_2$ ,  $\mathbf{r}_2 \sim \mathcal{U}(\mathbf{0}, \mathbf{1})$ ;
         $\mathbf{v}_j^{(i+1)} \leftarrow \omega \mathbf{v}_j^{(i)} + \left( \mathbf{p}_j^{(i)} - \mathbf{x}_j^{(i)} \right) \odot \phi_1 + \left( \mathbf{g}^{(i)} - \mathbf{x}_j^{(i)} \right) \odot \phi_2$ ;
        // Clamp the sampled positions to the discrete feature space
         $\mathbf{x}_j^{(i+1)} \leftarrow \arg \min_{\mathbf{x}_k \in \mathcal{X}} \left( \left\| \mathbf{x}_j^{(i)} + \mathbf{v}_j^{(i+1)} - \mathbf{x}_k \right\|_2 \right)$ ;

    // Evaluate positions using objective function f
     $\mathbf{g}^{(i+1)} \leftarrow \mathbf{g}^{(i)}$ ;
    for  $j \leftarrow 1$  to  $n_p$  do
        if  $s\left(\mathbf{f}\left(\mathbf{x}_j^{(i+1)}\right)\right) \geq s\left(\mathbf{f}\left(\mathbf{p}_j^{(i)}\right)\right)$  then
             $\mathbf{p}_j^{(i+1)} \leftarrow \mathbf{x}_j^{(i+1)}$ 
        else
             $\mathbf{p}_j^{(i+1)} \leftarrow \mathbf{p}_j^{(i)}$ 
        if  $s\left(\mathbf{f}\left(\mathbf{x}_j^{(i+1)}\right)\right) \geq s\left(\mathbf{f}\left(\mathbf{g}^{(i+1)}\right)\right)$  then
             $\mathbf{g}^{(i+1)} \leftarrow \mathbf{x}_j^{(i+1)}$ 
```

---

In [Algorithm 1](#), we initialise particle positions using a low-discrepancy Sobol sequence [15] ( $\mathcal{LDS}$ ) to maximise coverage of the search space. The velocities are initialised to zero. For chemical reaction optimisation, we systematically clamp the initialised positions  $\mathbf{x}_j^0$  to the valid search space  $\mathcal{X}$  with  $\arg \min_{\mathbf{x}_k \in \mathcal{X}} (\|\mathbf{x}_j - \mathbf{x}_k\|_2)$ . This clamping procedure is necessary because chemical reaction optimisation involves discrete and categorical variables (catalysts, solvents, bases, etc.) that define a finite set of valid experimental conditions. Unlike continuous optimisation problems where the search space spans all of  $\mathbb{R}^d$ , the featurised reaction search space  $\mathcal{X}$  consists only of defined reaction condition combinations. If a particle is moved to a non-defined position  $\mathbf{x}_p \notin \mathcal{X}$ , we map it to the nearest valid

experimental condition using  $\arg \min_{\mathbf{x}_k \in \mathcal{X}} (\|\mathbf{x}_p - \mathbf{x}_k\|_2) \in \mathcal{X}$ . Next, we introduce our ML-augmented extension of PSO,  $\alpha$ -PSO, in [Algorithm 2](#).

### 2.3 $\alpha$ -PSO: Machine learning-augmented PSO

We extend canonical PSO to  $\alpha$ -PSO ([Algorithm 2](#)) by augmenting the velocity update mechanisms of each particle with ML predictive guidance. Unlike existing methods which use surrogate models to directly guide particles [\[21\]](#), we use batched Bayesian optimisation acquisition functions, complementing the desired balance of explorative and exploitative optimisation behaviour inherent to swarm intelligence. We enhance the traditional two-term velocity update in canonical PSO (Equation [2](#)) with a third ML influence term:

$$\mathbf{v}_j^{(i+1)} = \omega \mathbf{v}_j^{(i)} + \left( \mathbf{p}_j^{(i)} - \mathbf{x}_j^{(i)} \right) \odot \phi_1 + \left( \mathbf{g}^{(i)} - \mathbf{x}_j^{(i)} \right) \odot \phi_2 + \left( \hat{\mathbf{a}}_j^{(i)} - \mathbf{x}_j^{(i)} \right) \odot \phi_a \quad (4)$$

$$\mathbf{x}_j^{(i+1)} = \mathbf{x}_j^{(i)} + \mathbf{v}_j^{(i+1)} \quad (5)$$

Where  $\phi_a = c_{\text{ml}} \mathbf{r}_a$ ,  $\mathbf{r}_a \sim \mathcal{U}(\mathbf{0}, \mathbf{1})$  is a random vector sampled from a uniform distribution, and  $c_{\text{ml}} \in \mathbb{R}$  is the coefficient weighting the amount of ML guidance. We define the promising ML predicted positions  $\hat{\mathbf{a}}_j^{(i)}$  as the position  $\mathbf{x} \in \mathcal{X}$  with the  $j^{\text{th}}$  highest acquisition function value, where  $\hat{\mathbf{a}}_j^{(i)}$  corresponds to the  $j$ -th ranked position when all  $\mathbf{x} \in \mathcal{X}$  are ordered by  $\hat{\alpha}(\mathbf{x})$  in descending order, with particle  $j$  receiving guidance from  $\hat{\mathbf{a}}_j^{(i)}$ . Here,  $\hat{\alpha}(\mathbf{x})$  is a batched multi-objective Bayesian optimisation acquisition function which quantifies the utility of evaluating position  $\mathbf{x} \in \mathcal{X}$  based on all currently evaluated positions (obtained experimental data). In our implementation of  $\alpha$ -PSO, we used the qNEHVI acquisition function [\[3\]](#) for  $\hat{\alpha}(\mathbf{x})$ . To assist particles stuck in poorly performing regions,  $\alpha$ -PSO also optionally relocates the  $n_{\text{worst}}$  poorest-performing particles directly to  $\hat{\alpha}(\mathbf{x})$  maxima:  $\mathbf{x}_j^{(i+1)} = \hat{\mathbf{a}}_j^{(i)}$  for  $j \in \{\text{worst } n_{\text{worst}} \text{ particles}\}$ .  $\alpha$ -PSO provides a smooth transition between pure meta-heuristic optimisation and black box ML-driven search, offering a powerful yet comprehensible framework that bridges the performance of sophisticated ML methods with methodological clarity for scientific discovery.



---

**Algorithm 2:**  $\alpha$ -PSO - Machine learning-guided Particle Swarm Optimisation Algorithm

---

**Input :**  $\mathcal{X}$ , a normalised feature search space,  $\mathbf{f} : \mathcal{X} \rightarrow \mathbb{R}^m$ , an objective function with  $m$  objectives,  $\left\{q_j = \left(\mathbf{x}_j^{(i)}, \mathbf{v}_j^{(i)}, \mathbf{p}_j^{(i)}\right)\right\}_{j=1}^{n_p}$ , a set of  $n_p$  particles,  $c_1 \in \mathbb{R}$ , a cognitive parameter,  $c_2 \in \mathbb{R}$ , a social parameter,  $c_{ml} \in \mathbb{R}$ , a coefficient for weighting ML guidance,  $\omega \in \mathbb{R}$ , an inertia weight,  $n_i$ , the number of iterations,  $n_p$ , the number of particles forming the swarm,  $\mathbf{s} : \mathbb{R}^m \rightarrow \mathbb{R}$ , a scalarisation function combining multiple objectives into a single score,  $\{\boldsymbol{\alpha}_j^{(i)}\}_{j=1}^{n_p}$ , ML predictions of promising positions for each particle  $j$  at iteration  $i$ ,  $d \in \mathbb{N}$ , the dimensionality of the search space.

**Output:** An approximate global best position  $\mathbf{g}$  that maximises  $\mathbf{f}$ .

```

/* Initialisation of the particles                                     */
for  $j \leftarrow 1$  to  $n_p$  do
     $\mathbf{x}_j^{(0)} \leftarrow \arg \min_{\mathbf{x}_k \in \mathcal{X}} \left( \|\mathbf{x}_j^0 - \mathbf{x}_k\|_2 \right), \quad \mathbf{x}_j^0 \sim \mathcal{LDS}(d, j);$ 
     $\mathbf{p}_j^{(0)} \leftarrow \mathbf{x}_j^{(0)};$ 
     $\mathbf{v}_j^{(0)} \leftarrow \mathbf{0};$ 
/* Evaluate positions using objective function f                       */
 $j^* \leftarrow \arg \max_j s(\mathbf{f}(\mathbf{x}_j^{(0)}));$ 
 $\mathbf{g}^{(0)} \leftarrow \mathbf{x}_{j^*}^{(0)};$ 
/* Optimisation loop                                                 */
for  $i \leftarrow 0$  to  $n_i - 1$  do
    for  $j \leftarrow 1$  to  $n_p$  do
         $\phi_1 \leftarrow c_1 \mathbf{r}_1, \quad \mathbf{r}_1 \sim \mathcal{U}(\mathbf{0}, \mathbf{1});$ 
         $\phi_2 \leftarrow c_2 \mathbf{r}_2, \quad \mathbf{r}_2 \sim \mathcal{U}(\mathbf{0}, \mathbf{1});$ 
         $\phi_\alpha \leftarrow c_{ml} \mathbf{r}_a, \quad \mathbf{r}_a \sim \mathcal{U}(\mathbf{0}, \mathbf{1});$ 
         $\mathbf{v}_j^{(i+1)} \leftarrow \omega \mathbf{v}_j^{(i)} + \left( \mathbf{p}_j^{(i)} - \mathbf{x}_j^{(i)} \right) \odot \phi_1 + \left( \mathbf{g}^{(i)} - \mathbf{x}_j^{(i)} \right) \odot \phi_2 + \left( \boldsymbol{\alpha}_j^{(i)} - \mathbf{x}_j^{(i)} \right) \odot \phi_\alpha;$ 
        // Clamp the position to the feature space
         $\mathbf{x}_j^{(i+1)} \leftarrow \arg \min_{\mathbf{x}_k \in \mathcal{X}} \left( \left\| \mathbf{x}_j^{(i)} + \mathbf{v}_j^{(i+1)} - \mathbf{x}_k \right\|_2 \right);$ 
    // Evaluate positions using objective function f
     $\mathbf{g}^{(i+1)} \leftarrow \mathbf{g}^{(i)};$ 
    for  $j \leftarrow 1$  to  $n_p$  do
        if  $s\left(\mathbf{f}\left(\mathbf{x}_j^{(i+1)}\right)\right) \geq s\left(\mathbf{f}\left(\mathbf{p}_j^{(i)}\right)\right)$  then
             $\mathbf{p}_j^{(i+1)} \leftarrow \mathbf{x}_j^{(i+1)}$ 
        else
             $\mathbf{p}_j^{(i+1)} \leftarrow \mathbf{p}_j^{(i)}$ 
        if  $s\left(\mathbf{f}\left(\mathbf{x}_j^{(i+1)}\right)\right) \geq s\left(\mathbf{f}\left(\mathbf{g}^{(i+1)}\right)\right)$  then
             $\mathbf{g}^{(i+1)} \leftarrow \mathbf{x}_j^{(i+1)}$ 

```

---

### 3 Emulated benchmark datasets

#### 3.1 Creating virtual benchmarks with experimental data

To assess and compare reaction optimisation methods, we required chemically significant reaction benchmarks that reflect real-world reaction optimisation challenges. Existing reaction datasets and virtual benchmarks from the literature generally explore limited reaction condition spaces with few categorical variables (e.g., ligands, solvents, and bases) for a given substrate combination. These narrow scopes fail to capture the complexity and scale of real-world large-scale high-throughput experimentation (HTE) reaction optimisation campaigns. [5, 22, 23]. We therefore developed more comprehensive benchmarks using in-house experimental data from two HTE optimisation campaigns: a Ni-catalysed Suzuki reaction (576 reactions) and a Pd-catalysed Buchwald-Hartwig coupling (384 reactions) of an active pharmaceutical ingredient (API) [5]. The resulting virtual benchmarks comprised 87,203 reactions for the Ni-catalysed Suzuki reaction and 38,610 reactions for the Pd-catalysed Buchwald-Hartwig coupling.

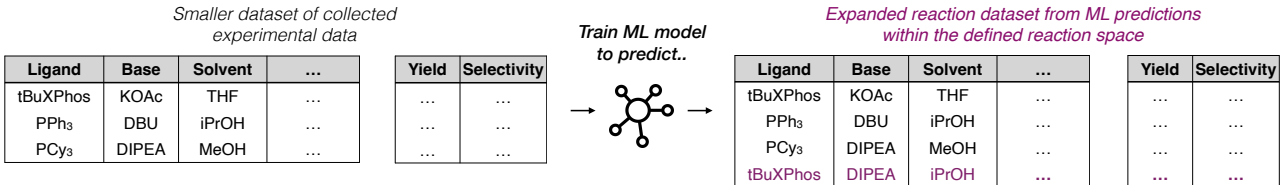

**Supplementary Figure 2:** Workflow for generating virtual benchmarks from experimental data.

For both datasets, we used regression models to predict reaction yields and selectivities for unexplored reaction conditions within the defined reaction spaces (Supplementary Figure 2). After evaluating Ridge, Lasso, and multilayer perceptron (MLP) regressors, we selected the MLP regressor based on superior performance in 5-fold cross-validation as measured by mean squared error. The MLP hyperparameters were optimised through grid search (Table 1). All models were implemented in scikit-learn [24] using normalised reaction features and standardised AP yield and selectivity values as targets. To ensure chemically meaningful predictions, we bounded predictions between 0-100%. Reactions with predicted yields below 5% had both yield and selectivity values set to 0%, and we removed predictions where yield exceeded selectivity to reflect physically impossible predictions. The complete virtual benchmark datasets are available in the GitHub repository accompanying this manuscript.

**Supplementary Table 1:** Hyperparameter grid search space for MLP.

| Hyperparameter              | Values                                                    |
|-----------------------------|-----------------------------------------------------------|
| Hidden layer sizes          | {(50,), (100,), (150,), (50, 50), (100, 100), (150, 150)} |
| Maximum iterations          | {1000, 1500}                                              |
| Regularisation ( $\alpha$ ) | {0.0001, 0.001, 0.01}                                     |

#### 3.2 Analysing reaction landscape topology with local Lipschitz constants

Sharp changes in yield and selectivity with respect to minute changes in reaction conditions are often observed in chemical reactions, resulting in reactivity cliffs: regions where small modifications in, for example, ligand structure, temperature, or solvent can substantially alter reaction outcomes, creating discontinuous and less predictable experimental landscapes. The presence and frequency of reactivity cliffs affect the choice of optimisation strategy, with comparatively “rougher” and “smoother”

landscapes requiring different approaches. We used Lipschitz constants to quantify the steepness of the reaction landscape of the benchmark datasets, describing how “smooth” or “rough” experimental landscapes are. Local  $(\alpha, \beta)$ -Lipschitz constants are defined below.

**Definition 1.** The local  $(\alpha, \beta)$ -Lipschitz constant of a function  $\mathbf{f} : \mathcal{X} \rightarrow \mathcal{Z} \subseteq \mathbb{R}^m$  over the set  $\mathfrak{U} \subset \mathcal{X} \subset \mathbb{R}^d$  is defined as

$$L^{(\alpha, \beta)}(\mathbf{f}, \mathfrak{U}) = \sup_{\substack{\mathbf{x}, \mathbf{y} \in \mathfrak{U} \\ \mathbf{x} \neq \mathbf{y}}} \frac{\|\mathbf{f}(\mathbf{y}) - \mathbf{f}(\mathbf{x})\|_{\beta}}{\|\mathbf{y} - \mathbf{x}\|_{\alpha}} \quad (6)$$

where  $f(x)$  and  $f(y)$  represent reaction outcomes for the input conditions  $x$  and  $y$  in the benchmark dataset. If  $L^{(\alpha, \beta)}(\mathbf{f}, \mathfrak{U})$  exists and is finite, we say that  $\mathbf{f}$  is  $(\alpha, \beta)$ -locally Lipschitz over  $\mathfrak{U}$ .

We used the Euclidean norm to describe both the design space and objective space ( $\alpha = \beta = 2$  in Definition 1). This assumes that reaction conditions in the design space  $\mathcal{X}$  are similar when they are close in Euclidean space, and that this metric adequately captures meaningful chemical similarities. Our goal is to understand how predictably reaction outcomes (yield and selectivity) change when small adjustments are made to reaction conditions in the design space  $\mathcal{X}$ . To quantify this predictability, we compute local Lipschitz constants [25] using  $k$ -nearest neighbours [26]: for each reaction condition point in the design space, we identify its  $k$  closest neighbours and calculate the local Lipschitz constant among these points, quantifying how much the reaction outcomes change across its closest neighbours. Lower local Lipschitz constants indicate more predictable relationships between reaction conditions and outcomes, while higher values suggest that small changes in reaction conditions can lead to large, unpredictable changes in performance (reactivity cliffs). For fair comparisons between datasets with different feature dimensions, we normalise the local Lipschitz constants by  $\sqrt{d}$ , where  $d$  is the dimensionality of the chemical space  $\mathcal{X}$ . We compare the two benchmark datasets by examining the distribution of  $L^{(2,2)}(\mathbf{f}, \mathfrak{U})/\sqrt{d}$ . Supplementary Figure 3 shows the density distributions of normalised local Lipschitz constants of each reaction condition in our benchmark datasets across their 19 nearest neighbours. The distributions reveal that the Ni-Suzuki benchmark is significantly smoother than the Buchwald-Hartwig dataset. The Ni-Suzuki dataset shows consistently lower normalised local Lipschitz constants, with proportionally smaller and more predictable changes in yield and selectivity. In contrast, the Buchwald-Hartwig dataset exhibits much higher variability, with local Lipschitz constants reaching up to 2.5, four times higher than the maximum observed in the Ni-Suzuki dataset. This suggests that small changes to reaction conditions can cause large, unpredictable swings in performance, representing more reactivity cliffs and a more “rough” reaction landscape.

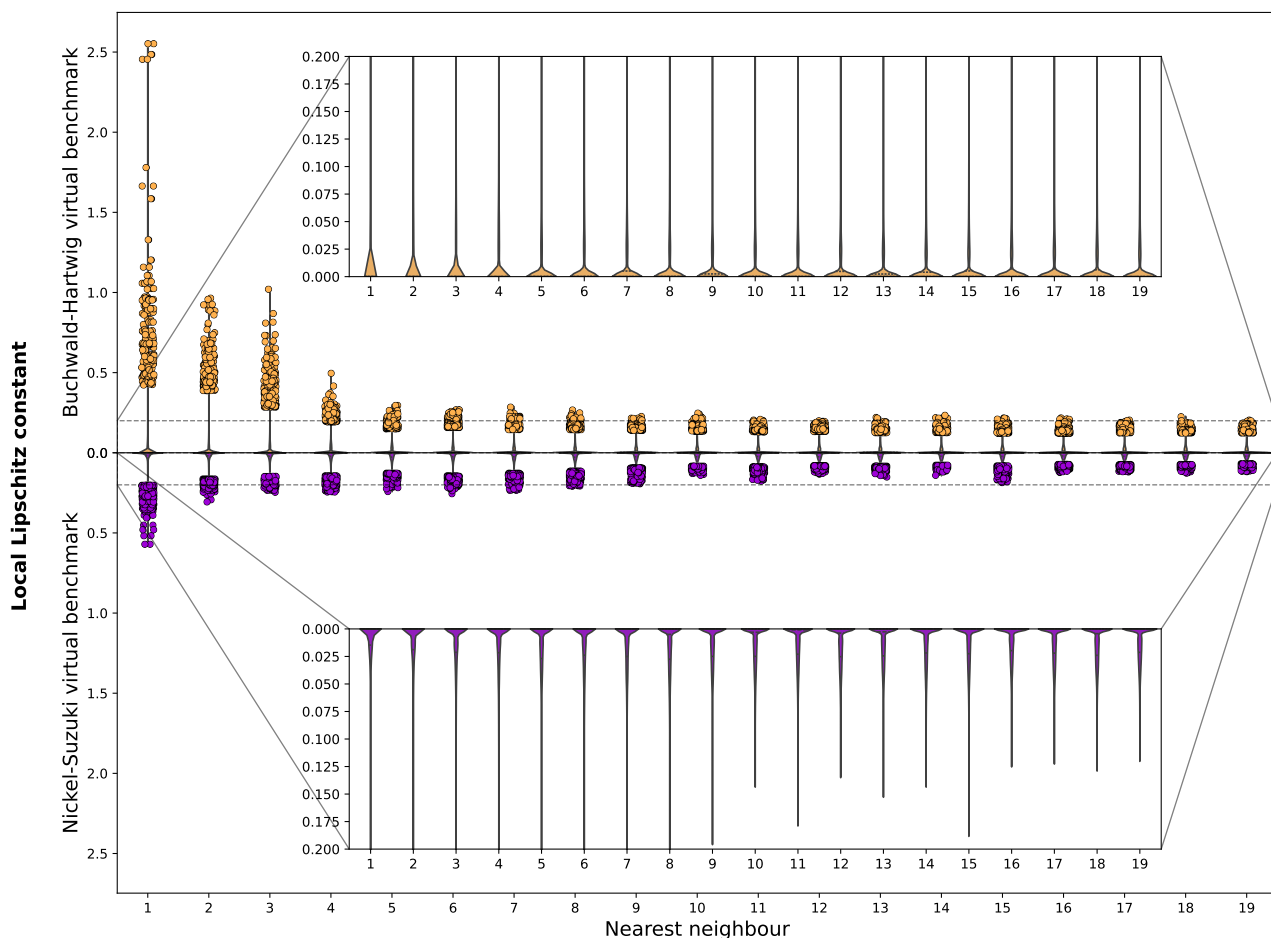

**Supplementary Figure 3: Comparison of reaction landscape smoothness between the two benchmark datasets.** Violin plots show the distribution of local Lipschitz constants of each reaction condition in the datasets across their  $k$ -closest neighbouring reaction conditions ( $k = 19$ ). Each data point in the distribution represents how much reaction condition outcomes change between their  $k^{th}$  closest neighbouring reaction conditions. Lower values indicate more predictable behaviour. Explicit data points are shown if they are above the 99.5th percentile to highlight extreme cases.

To further quantify the relative smoothness of these chemical reaction spaces, we analysed the distribution of normalised local Lipschitz constants across both datasets (Supplementary Figure 4). The Q-Q plot reveals distinct distribution characteristics between the two reaction types, corroborating our earlier analyses. The Ni-Suzuki dataset demonstrates a compact distribution with most Lipschitz constants concentrated at low values, indicating a smooth chemical space with predictable reactivity patterns. In contrast, the Buchwald-Hartwig dataset exhibits a pronounced tail extending to much higher Lipschitz constants, reaching values up to 2.5 compared to the Ni-Suzuki dataset’s maximum of approximately 0.6. This tail behaviour is quantified by substantially higher kurtosis (359.52 vs 14.94) values, indicating the presence of many high-value outliers. The pronounced tail represents a sharp increase in the frequency of high Lipschitz constant values, meaning that Buchwald-Hartwig contains more reactivity cliffs where small changes in reaction conditions produce disproportionately large changes in outcomes. The cumulative distribution plot shows a similar trend, with the Buchwald-Hartwig dataset exhibiting higher maximum Lipschitz constants and a more extended tail of extreme values compared to the more constrained Ni-Suzuki dataset distribution. These distributional differences have implications for optimisation algorithm performance, as the Buchwald-Hartwig landscape

with more reactivity cliffs presents a “rougher” optimisation landscape, while the Ni-Suzuki benchmark has a “smoother” variation in objective outcomes.

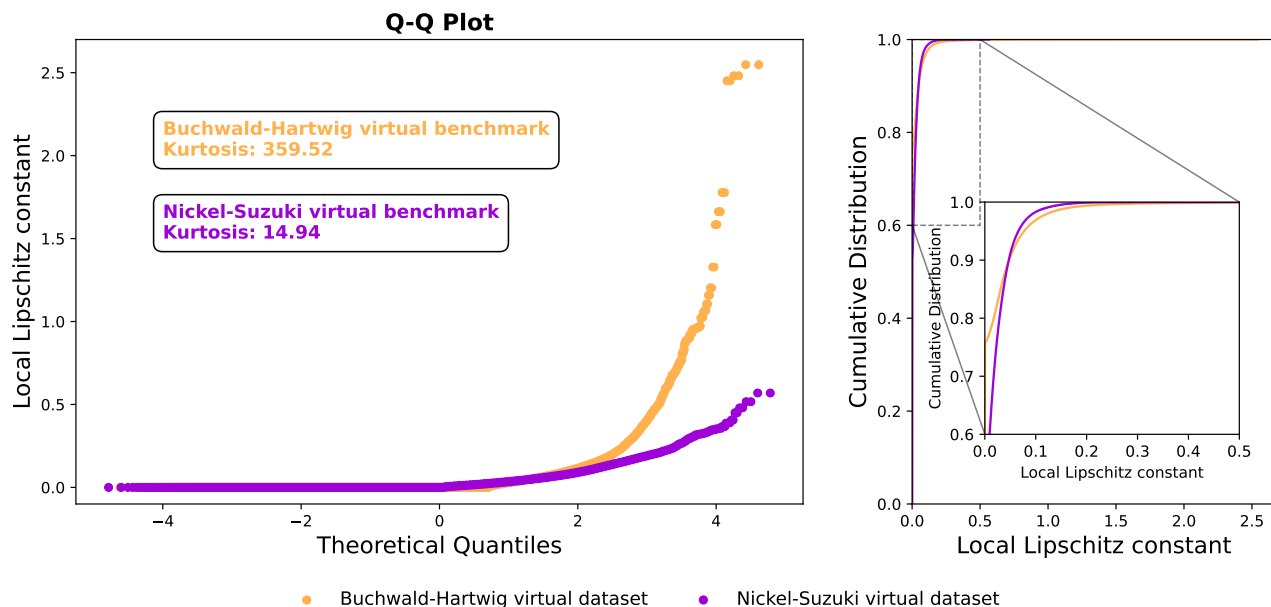

**Supplementary Figure 4: Distribution analysis of normalised local Lipschitz constants for the two benchmark datasets computed using  $k = 9$  nearest neighbours. Local Lipschitz constants were calculated by comparing each reaction condition to its 9 closest neighbours in the chemical space.** (Left) Q-Q plot comparing the distribution of normalised local Lipschitz constants between datasets. Each point represents the corresponding percentiles from both datasets. The x-axis shows theoretical quantiles from a standard normal distribution (representing expected percentile values if data were normally distributed with negative values representing lower percentiles and positive values representing higher percentiles), while the y-axis shows the actual Lipschitz constant values at corresponding percentiles in each dataset. Upward curves reveal heavy-tailed distributions containing extreme values. Statistical measures (kurtosis) quantify the degree of non-normality and tail heaviness in each benchmark dataset. (Right) Cumulative distribution functions showing the probability of encountering Lipschitz constants below given thresholds. The inset provides a detailed view of the 60th-100th percentile range.

In experimental campaigns, researchers often need to assess the characteristics of a chemical reaction space *a priori* before running extensive experiments. Our previous analysis (Supplementary Figures 3 and 4) demonstrated that when complete datasets are available, reaction space roughness can be characterised through local Lipschitz constant distributions, with the Buchwald-Hartwig benchmark dataset showing substantially higher roughness than the Ni-Suzuki benchmark dataset. However, this comprehensive assessment is not possible in real experimental scenarios where researchers must make strategic decisions based on limited initial data. While reaction roughness can be estimated through chemical intuition based on prior experimental experience, we hypothesise that quantitative roughness assessment of the entire reaction space can be achieved using only a small, well-designed initial sample of experiments. Given that quasi-random sequences like Sobol sampling [15] are designed for maximal space coverage, even limited experimental data sampled in this manner should provide meaningful insights into how objective responses vary across the chemical space. This led us to investigate whether a small subset of strategically sampled points can serve as a reliable predictor of overall reaction space characteristics, eliminating the need for complete experimental knowledge while maintaining predictive accuracy. To test this, we simulated virtual batches of 96 well experiments to mirror typical HTE

batch sizes, with each batch selected using Sobol sampling. To account for sampling randomness, we generated these batches at 20 different random seeds, creating multiple independent samples. For every data point in each virtual batch, we computed local Lipschitz constants using  $k = 9$  nearest neighbours, generating distributions of normalised local Lipschitz constants that quantify surface roughness. These distributions were then compared between datasets using Q-Q plots and cumulative distribution plots (Supplementary Figure 5) to assess whether small initial samples preserve the relative roughness characteristics observed in complete datasets.

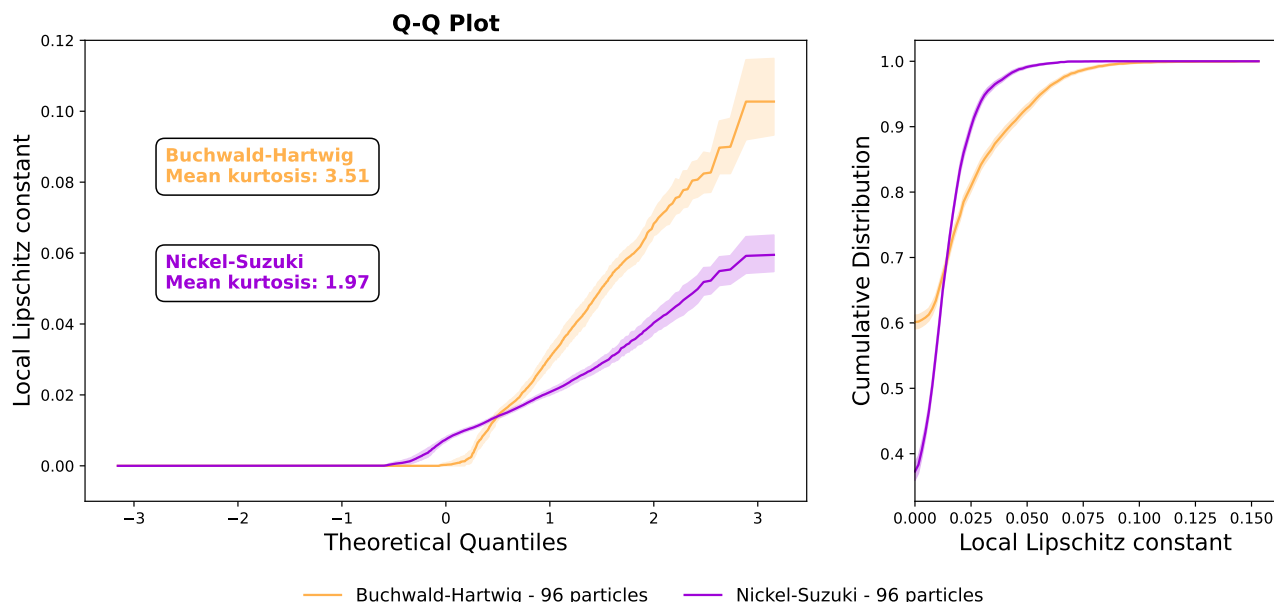

**Supplementary Figure 5: Assessment of complete reaction space roughness using limited initial sampling.** Distribution analysis of normalised local Lipschitz constants computed from virtual batches of 96 wells using  $k = 9$  nearest neighbours. Each batch was sampled 20 times with Sobol sequences using different random seeds to account for sampling variability, with confidence bands representing the distribution across these realisations. (Left) Q-Q plot comparing the distribution of normalised local Lipschitz constants between datasets. The x-axis shows theoretical quantiles from a standard normal distribution, while the y-axis shows the actual Lipschitz constant values at corresponding percentiles. Consistent upward separation between the orange (Buchwald-Hartwig) and purple (Ni-Suzuki) curves demonstrates the preservation of relative roughness characteristics. Statistical measures (mean kurtosis) averaged across all random seeds quantify the tail behaviour differences between datasets. (Right) Cumulative distribution functions showing the probability of encountering Lipschitz constants below given thresholds for each dataset. The consistent ordering between datasets across random seeds validates the reliability of early roughness assessment using strategically sampled initial experiments.

While these virtually subsampled batches contain only partial information about the complete experimental response surface, Supplementary Figure 5 demonstrates that it is possible to reliably distinguish between rough (Buchwald-Hartwig) and smooth (Ni-Suzuki) reaction surfaces even from limited sampling across many random seeds. The consistent separation between datasets across random realisations, with the Buchwald-Hartwig benchmark dataset showing systematically higher Lipschitz constants and greater tail behaviour (quantified by higher mean kurtosis: 3.51 vs 1.97), confirms that the relative roughness characteristics are preserved even in small samples. The confidence bands derived from 20 independent random seeds demonstrate the robustness of this distinction, with minimal overlap between the two datasets. However, the absolute magnitude of differences is substantially

compressed compared to full dataset analysis, with maximum Lipschitz constants reaching only 0.12 versus 2.5 in the complete datasets. These findings validate that strategically sampled initial batches can provide reliable early indicators of reaction space roughness, offering a practical framework for guiding subsequent experimental design decisions without requiring extensive prior experimentation.

## 4 Computational benchmarks

### 4.1 Baseline benchmarks

To evaluate the performance of the  $\alpha$ -PSO algorithm, we benchmarked it against three optimisation methods: (1) Bayesian optimisation using the Minerva workflow [5] with the qNEHVI [3] (q-Noisy Expected Hypervolume Improvement) acquisition function, which has demonstrated superior performance in Bayesian reaction optimisation over other approaches across multiple theoretical and empirical studies [3, 5, 27]; (2) The canonical PSO algorithm, following the implementation described in Algorithm 1; and (3) Quasi-random Sobol sampling [15] as a competitive baseline superior to pure random search. To establish a meaningful baseline performance for  $\alpha$ -PSO, we first evaluated its performance using default parameter settings with all coefficients set to unity ( $c_1 = c_2 = c_{ml} = 1.0$ ) without any tuning. This allowed us to isolate the core behavioural dynamics of  $\alpha$ -PSO under standardised conditions. We used the datasets described in Section 3.1 as benchmarks for optimisation. All optimisation methods were executed for six iterations in total, including initialisation. Batch sizes of 24, 48, and 96 were chosen to reflect commonly used plate sizes in high-throughput experimentation (HTE) platforms employing solid dosing. Each optimisation was repeated across 20 independent random seeds to ensure robust statistical comparison and account for stochasticity in the algorithms. Initial experiments for all algorithms were selected using Sobol sampling [15] to maximise coverage of the search space and increase the likelihood of capturing informative regions.

#### 4.1.1 Buchwald-Hartwig dataset

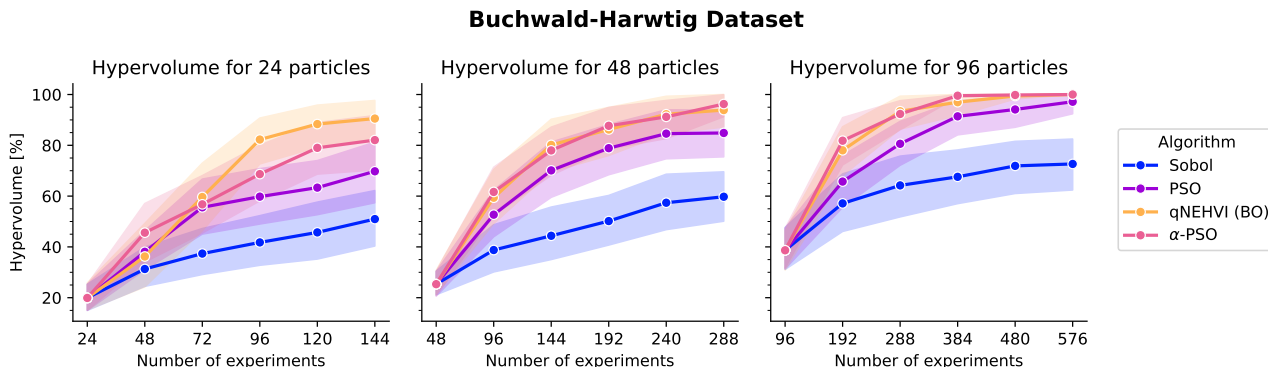

**Supplementary Figure 6:** Buchwald-Hartwig dataset baseline experiments. We compared the hypervolume (%) of the different optimisation algorithms across 20 random seeds and three batch sizes (24, 48, and 96). The shaded regions indicate the 95% confidence interval.



### 4.1.2 Ni-Suzuki dataset

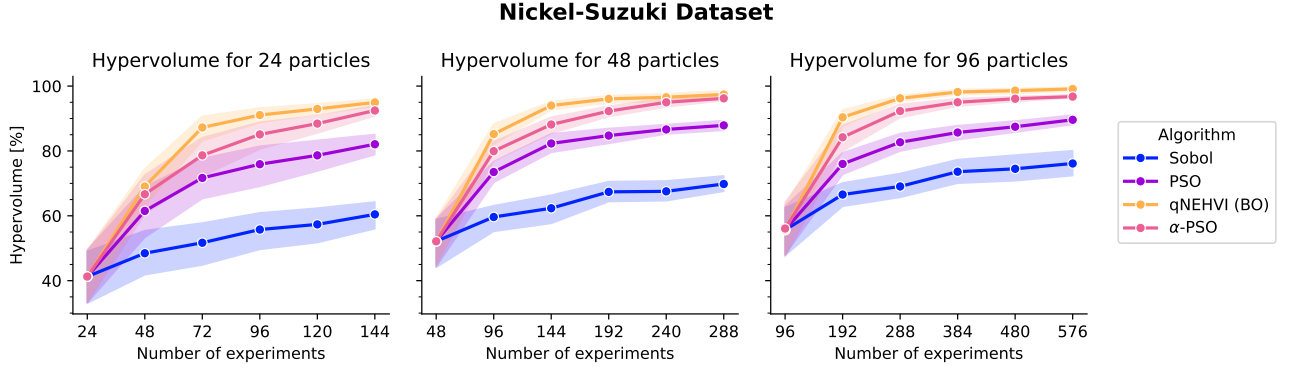

**Supplementary Figure 7:** Ni-Suzuki dataset baseline experiments. We compared the hypervolume (%) of the different optimisation algorithms across 20 random seeds and three batch sizes (24, 48, and 96). The shaded regions indicate the 95% confidence interval.

### 4.2 Effect of cognitive and social coefficients

To characterise the effect of  $\alpha$ -PSO hyperparameters, we performed a full grid search over the three  $\alpha$ -PSO coefficients controlling swarm behaviour: the cognitive coefficient  $c_1$ , the social coefficient  $c_2$ , and the ML coefficient  $c_{ml}$ . Each coefficient was swept over the set  $\{0.5, 1.0, 1.5, 2.0\}$ , yielding  $4^3 = 64$  parameter combinations.

### 4.2.1 Buchwald-Hartwig dataset

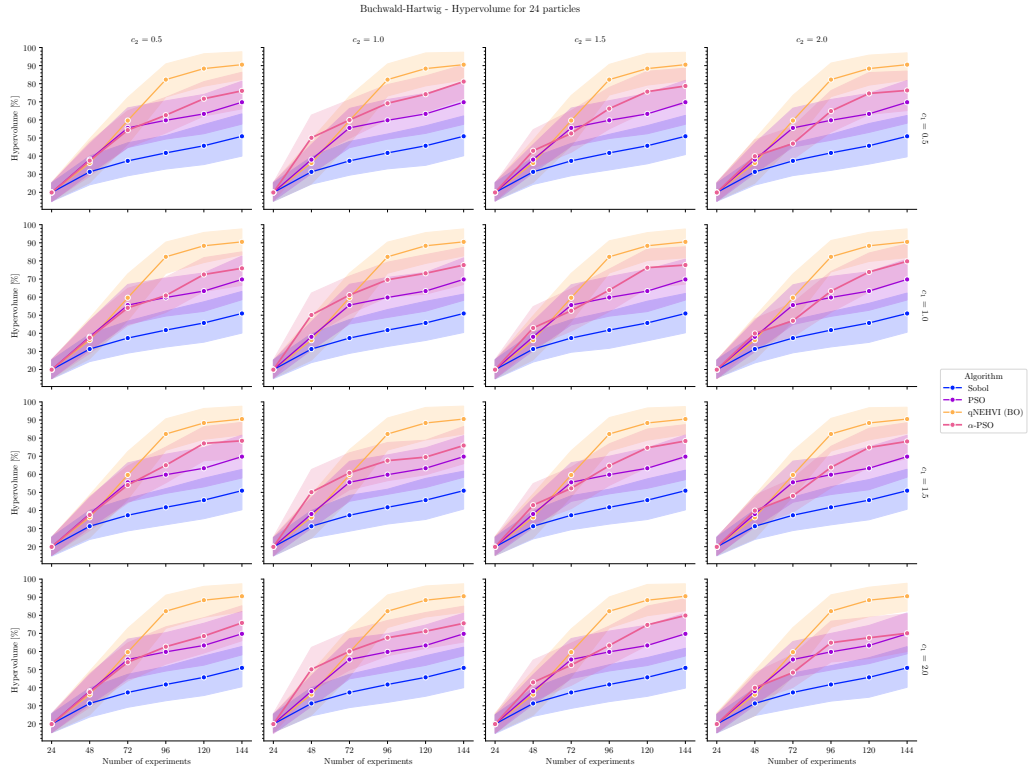

**Supplementary Figure 8:** Buchwald-Hartwig dataset, batch size 24,  $c_{ml} = 0.5$ .

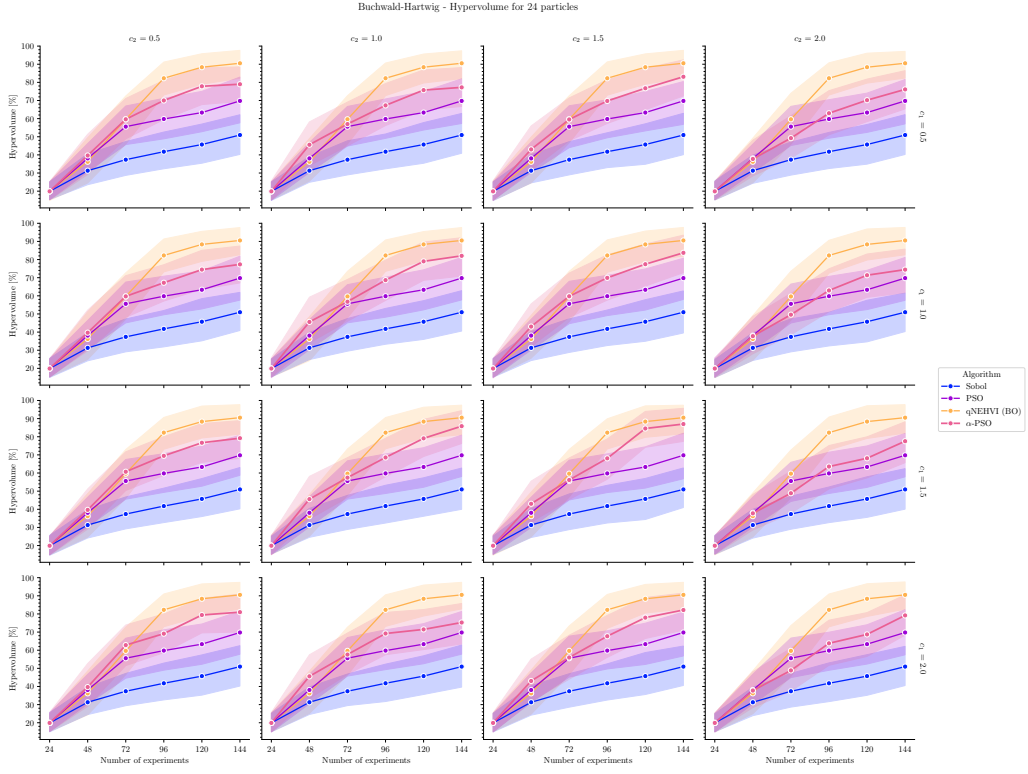

**Supplementary Figure 9:** Buchwald-Hartwig dataset, batch size 24,  $c_{ml} = 1.0$ .

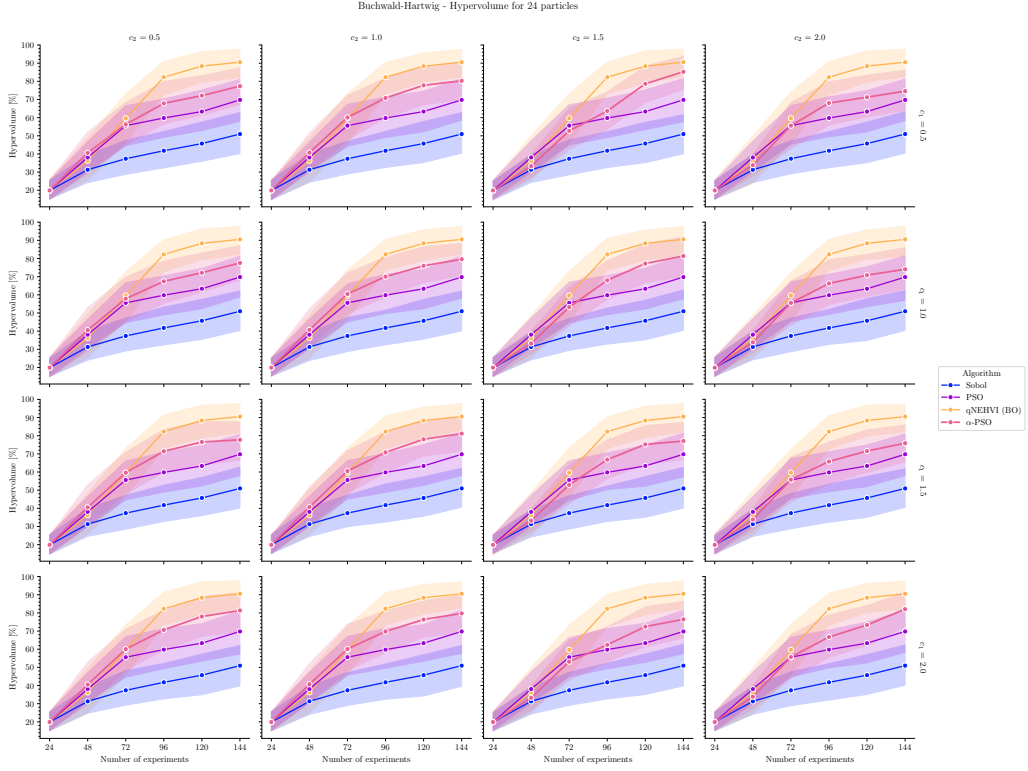

**Supplementary Figure 10:** Buchwald-Hartwig dataset, batch size 24,  $c_{ml} = 1.5$ .

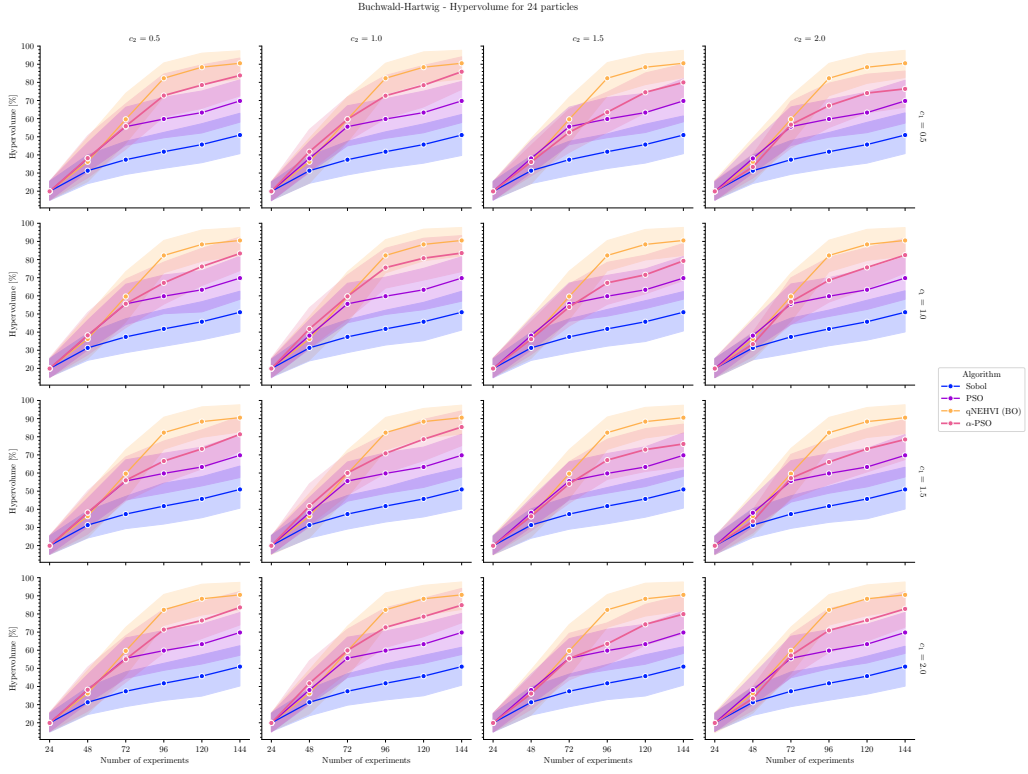

**Supplementary Figure 11:** Buchwald-Hartwig dataset, batch size 24,  $c_{ml} = 2.0$ .

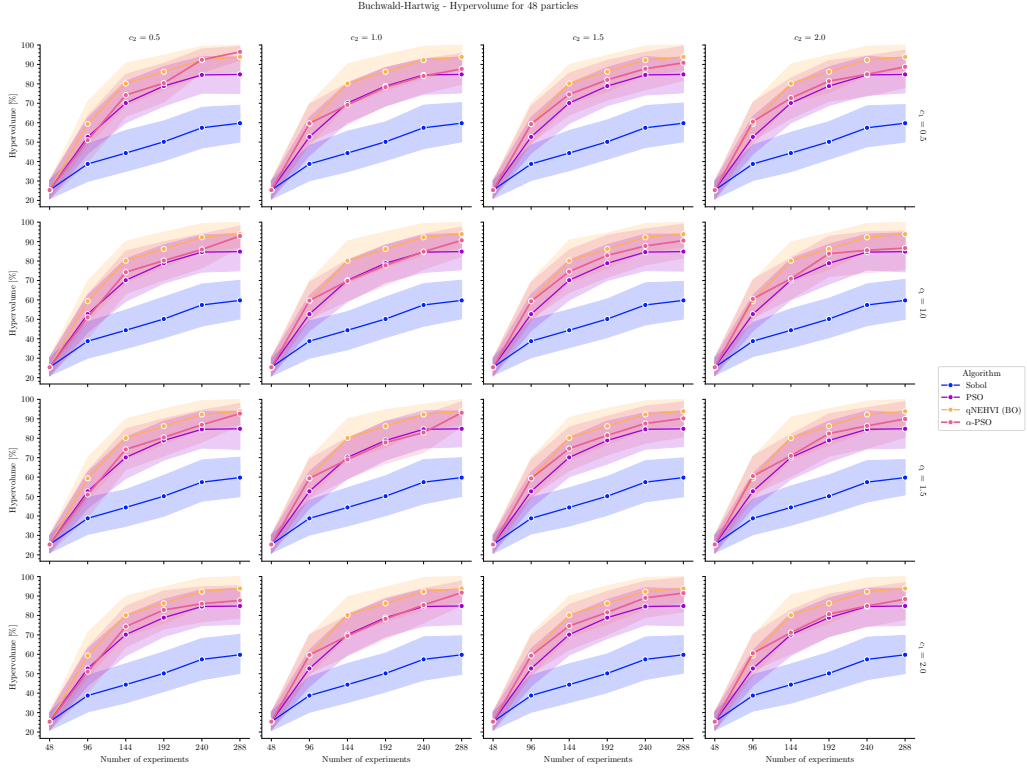

**Supplementary Figure 12:** Buchwald-Hartwig dataset, batch size 48,  $c_{ml} = 0.5$ .

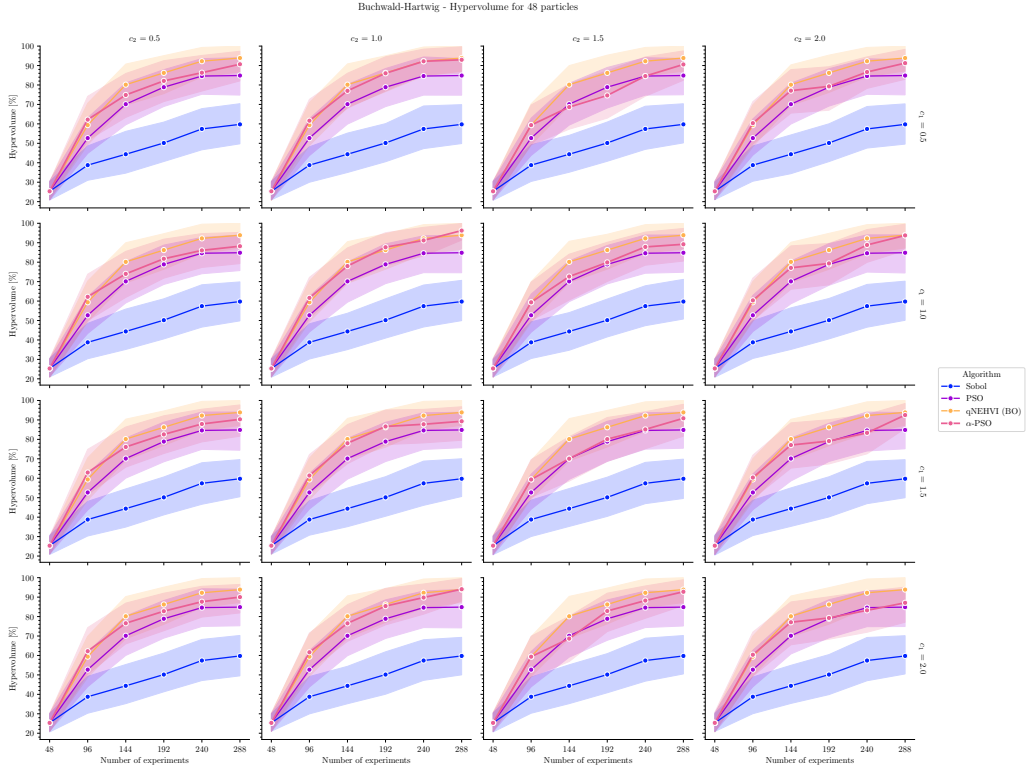

**Supplementary Figure 13:** Buchwald-Hartwig dataset, batch size 48,  $c_{ml} = 1.0$ .

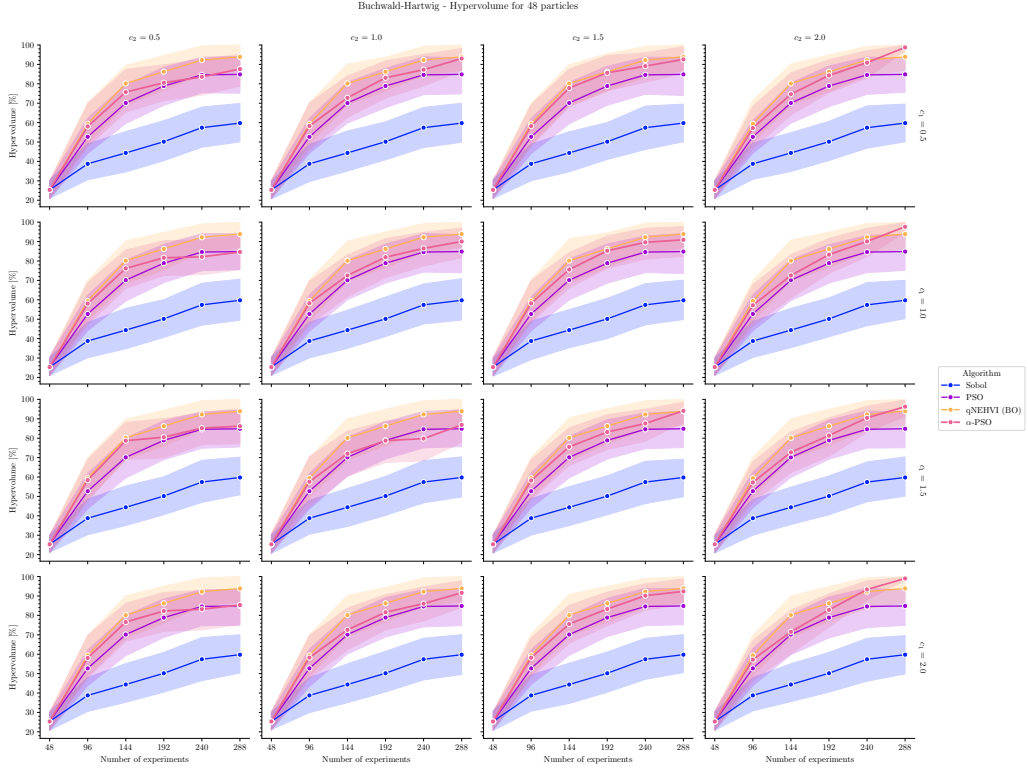

**Supplementary Figure 14:** Buchwald-Hartwig dataset, batch size 48,  $c_{ml} = 1.5$ .

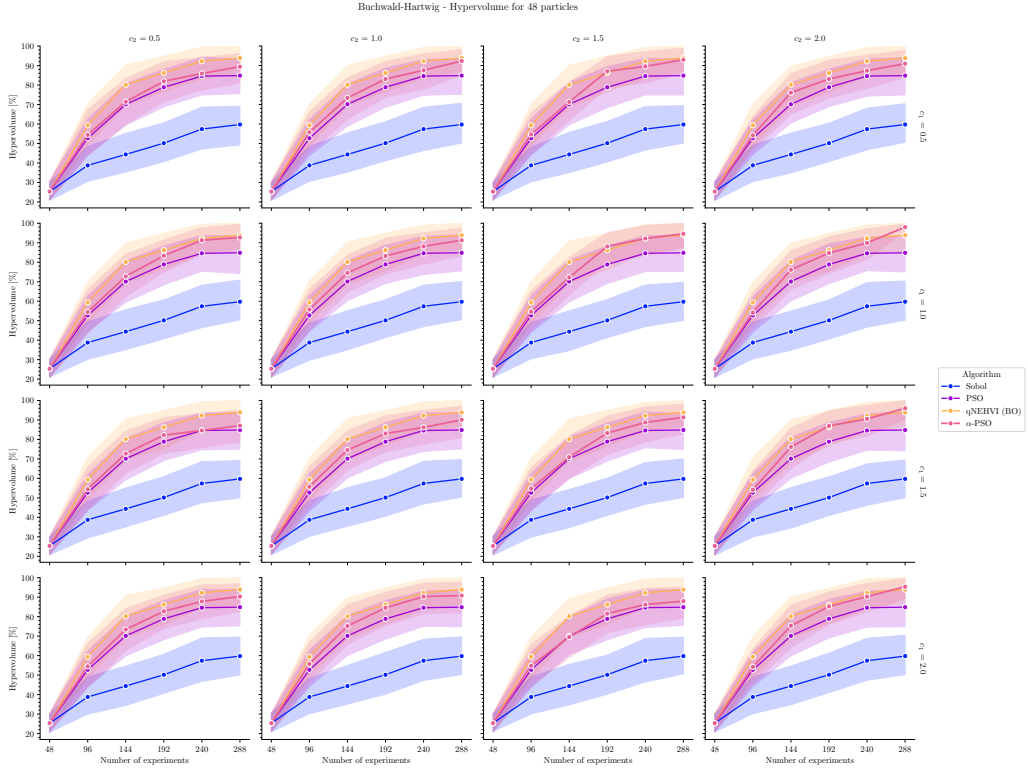

**Supplementary Figure 15:** Buchwald-Hartwig dataset, batch size 48,  $c_{ml} = 2.0$ .

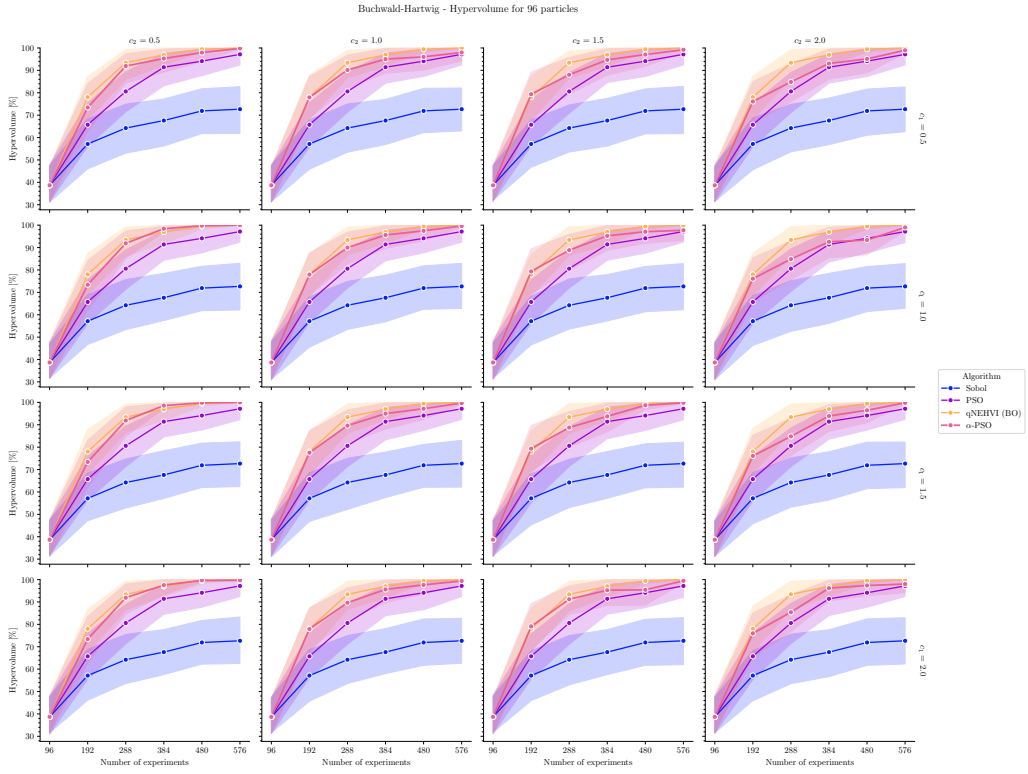

**Supplementary Figure 16:** Buchwald-Hartwig dataset, batch size 96,  $c_{ml} = 0.5$ .

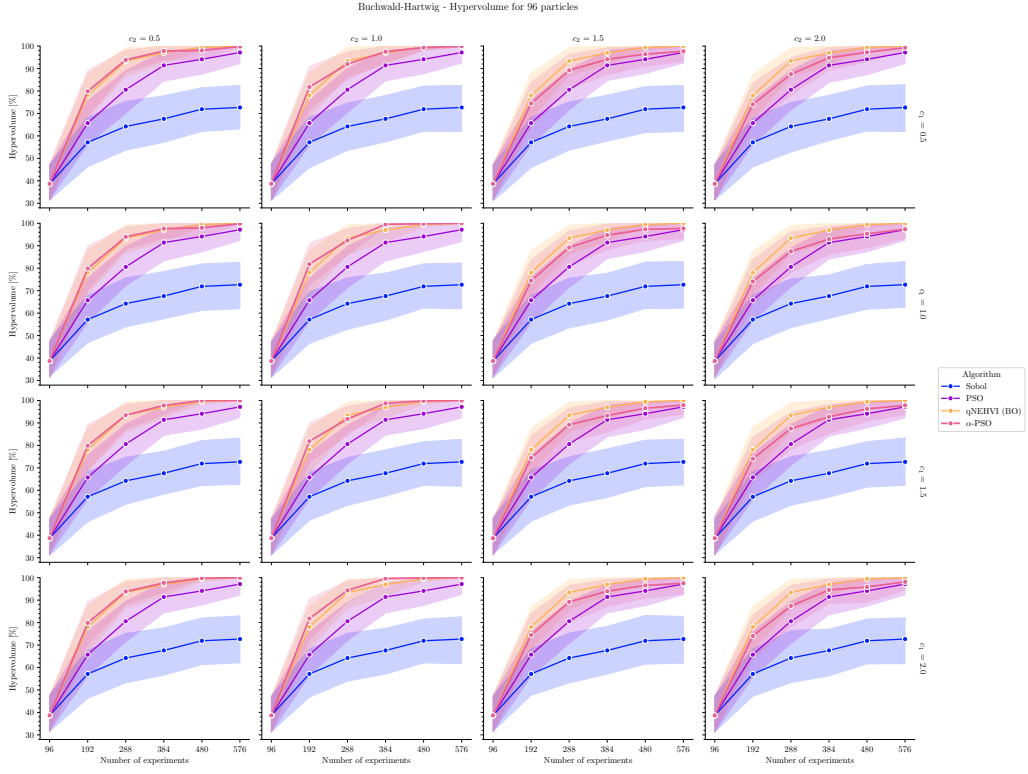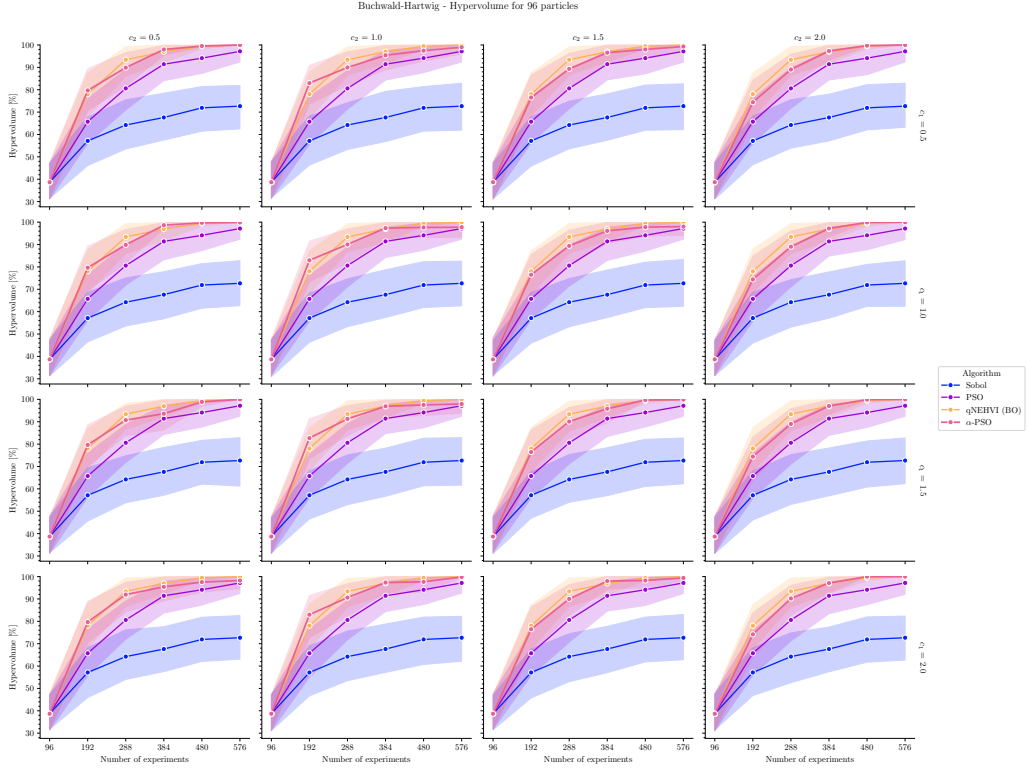

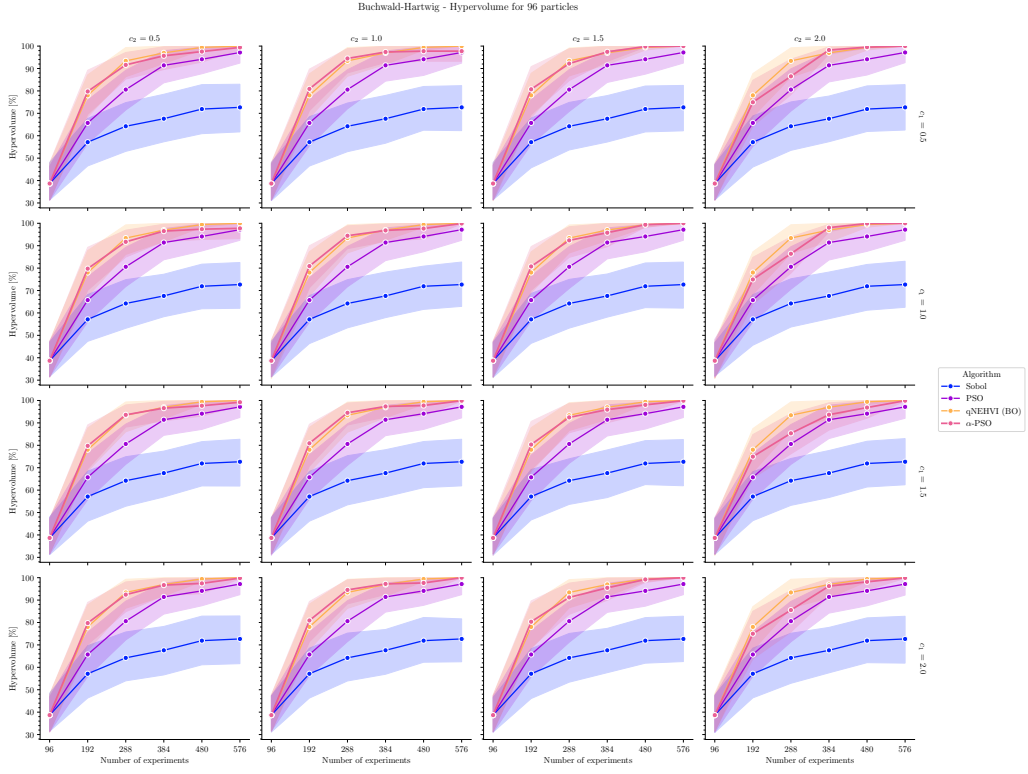

**Supplementary Figure 19:** Buchwald-Hartwig dataset, batch size 96,  $c_{ml} = 2.0$ .



## 4.2.2 Ni-Suzuki dataset

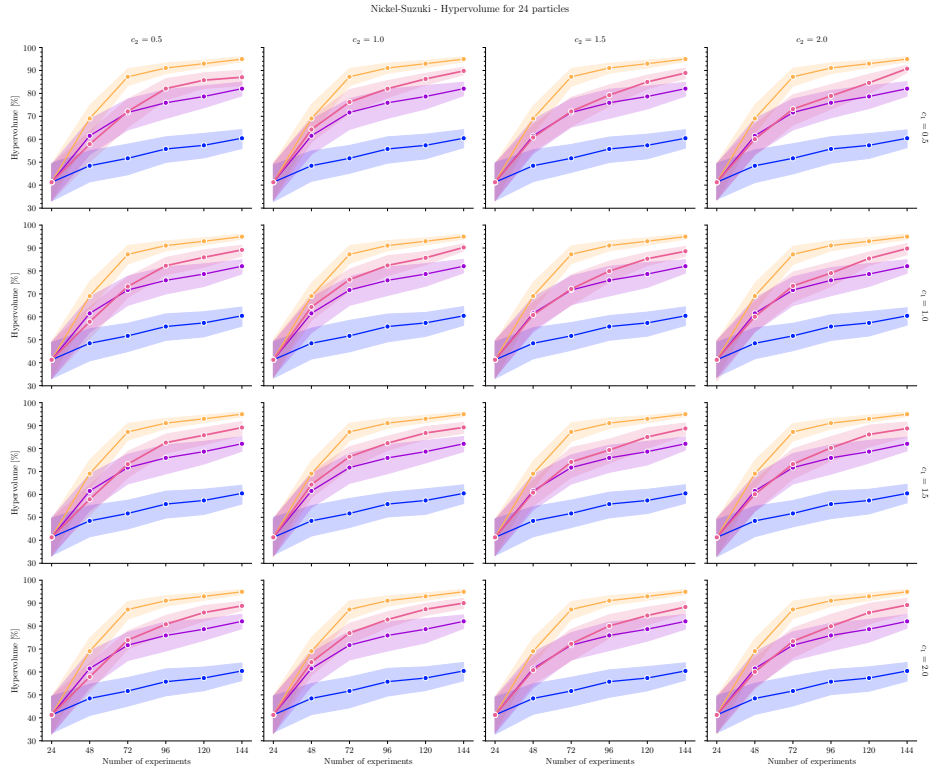

**Supplementary Figure 20:** Ni-Suzuki dataset, batch size 24,  $c_{ml} = 0.5$ .

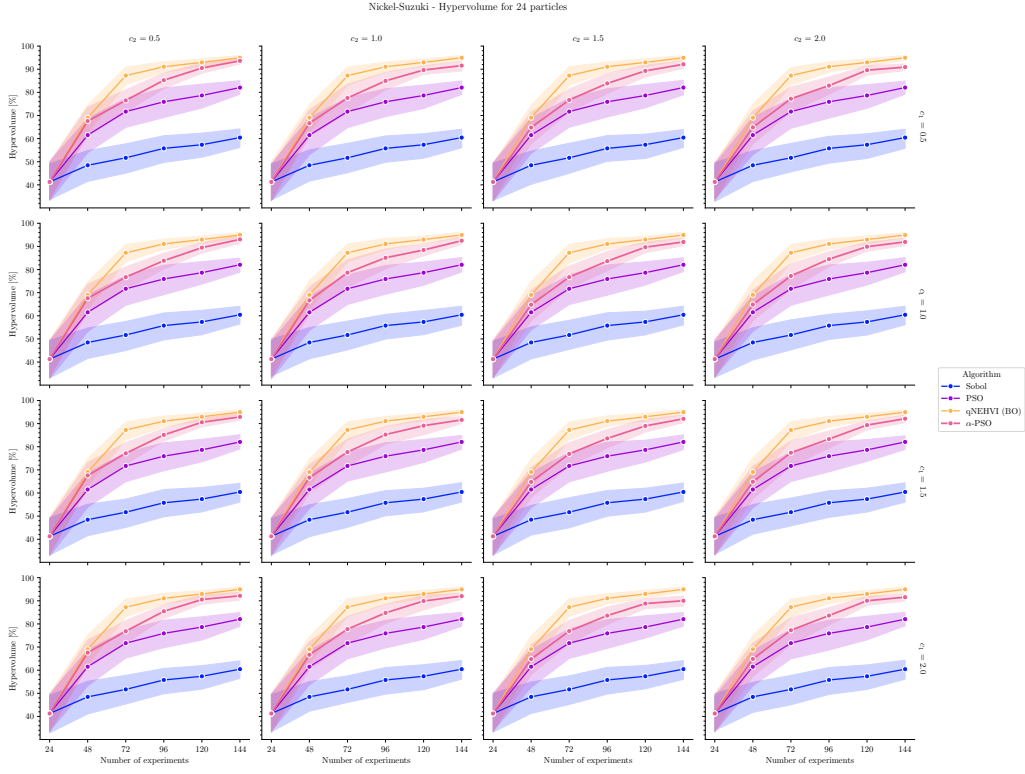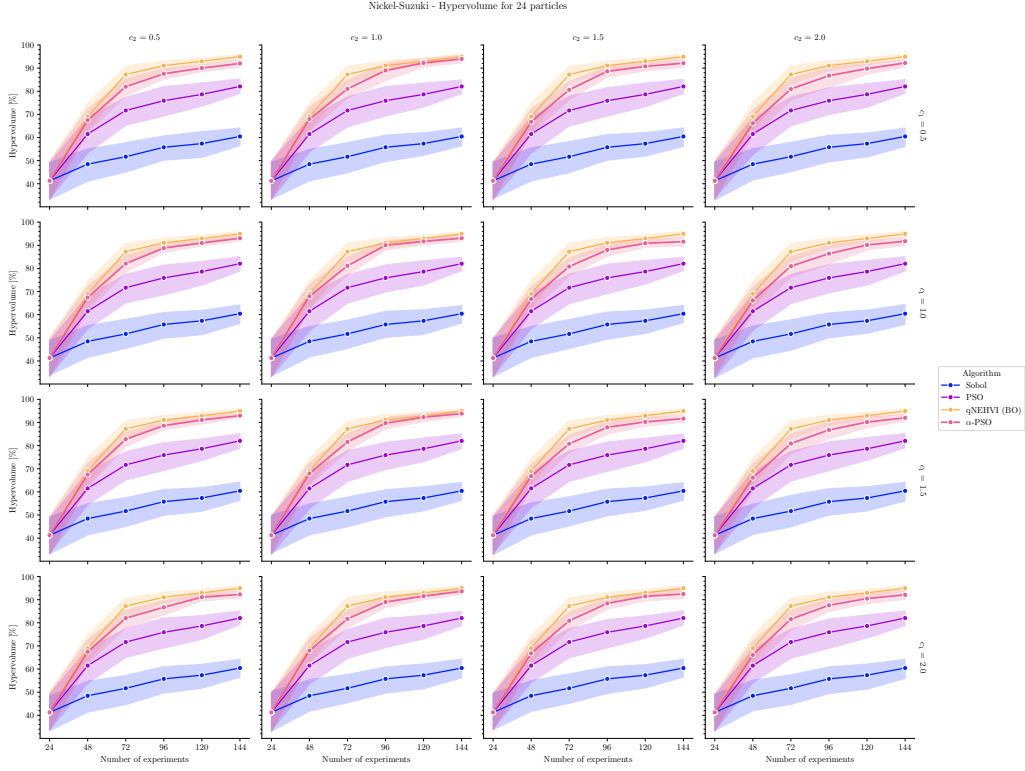

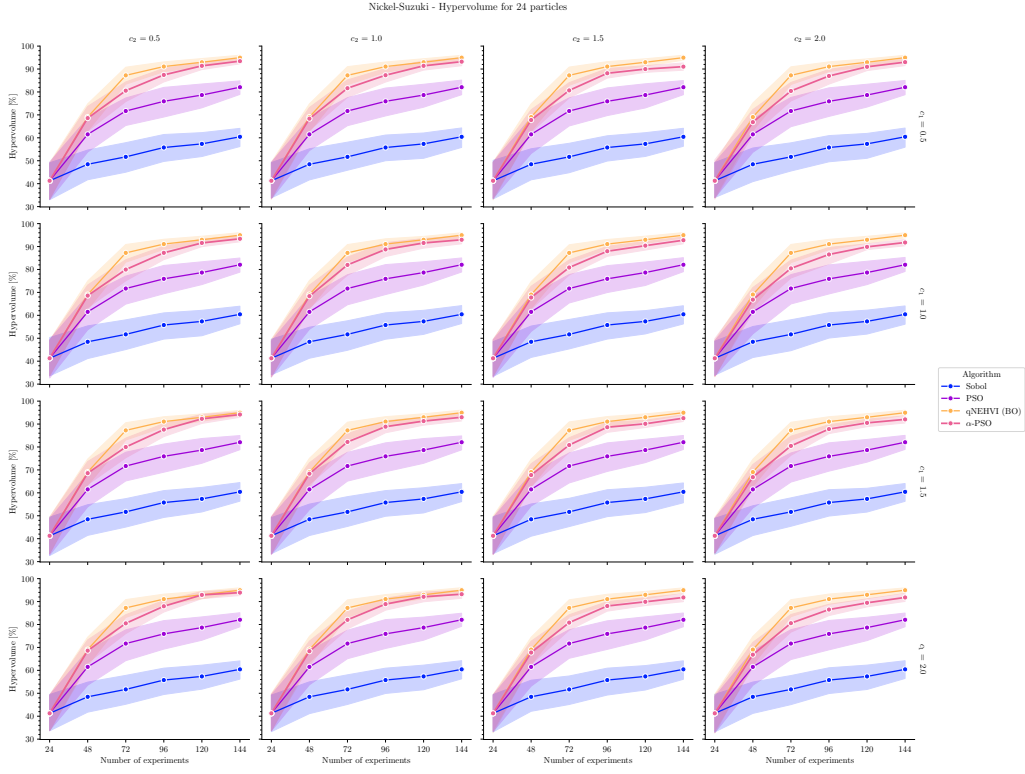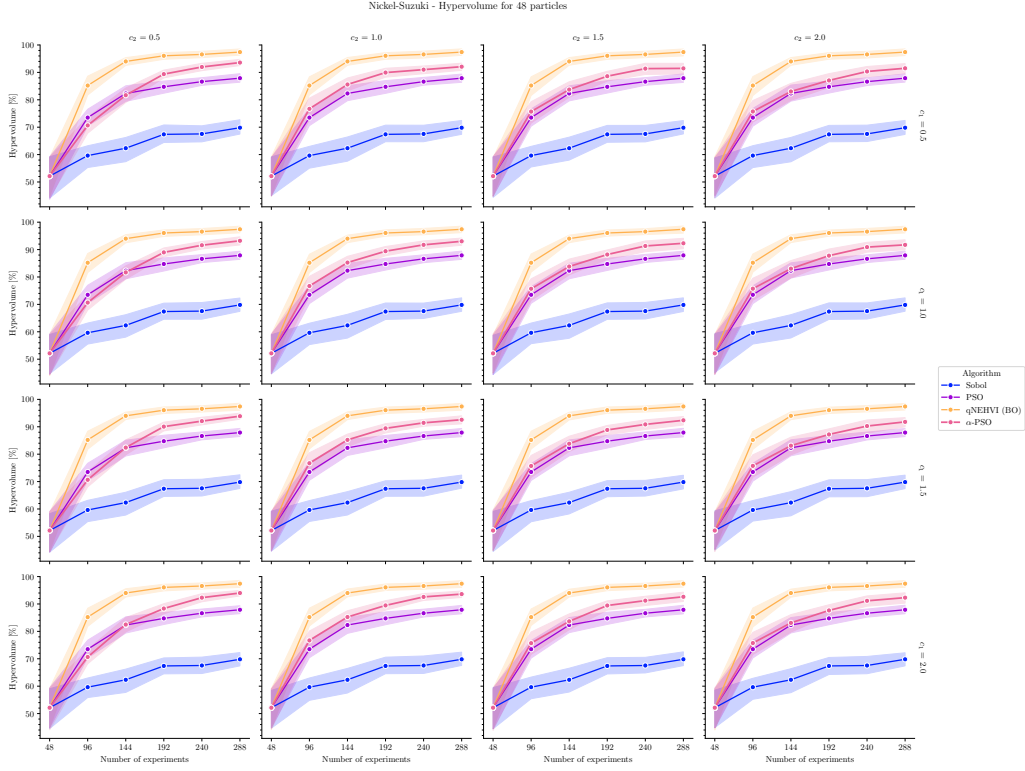

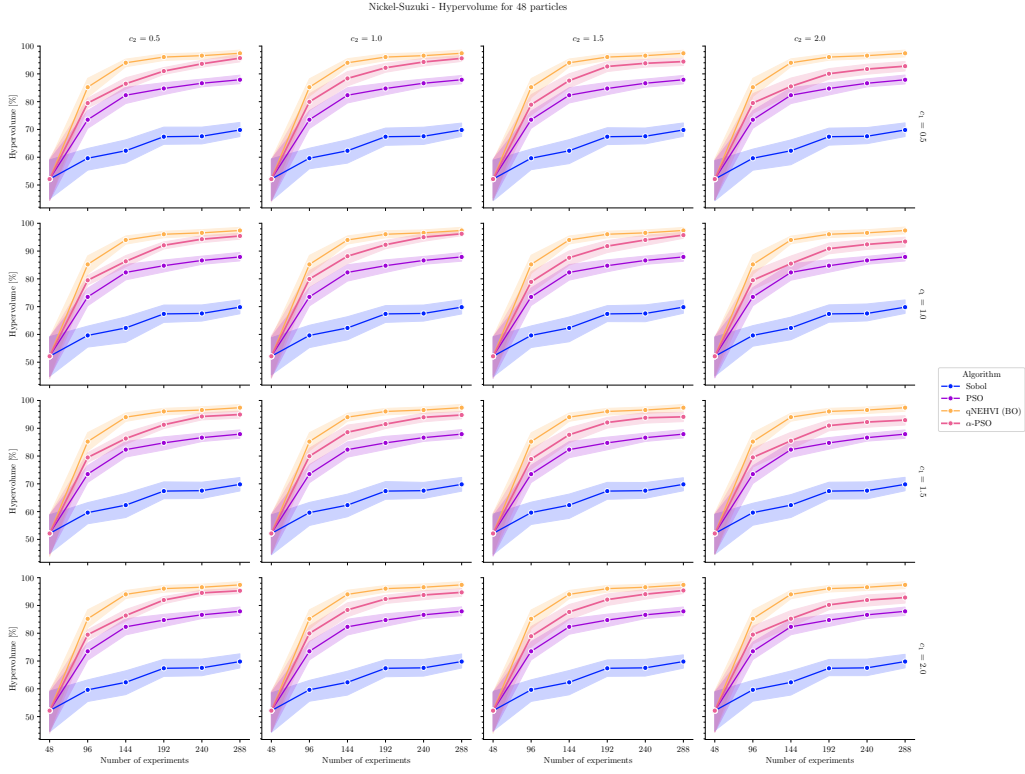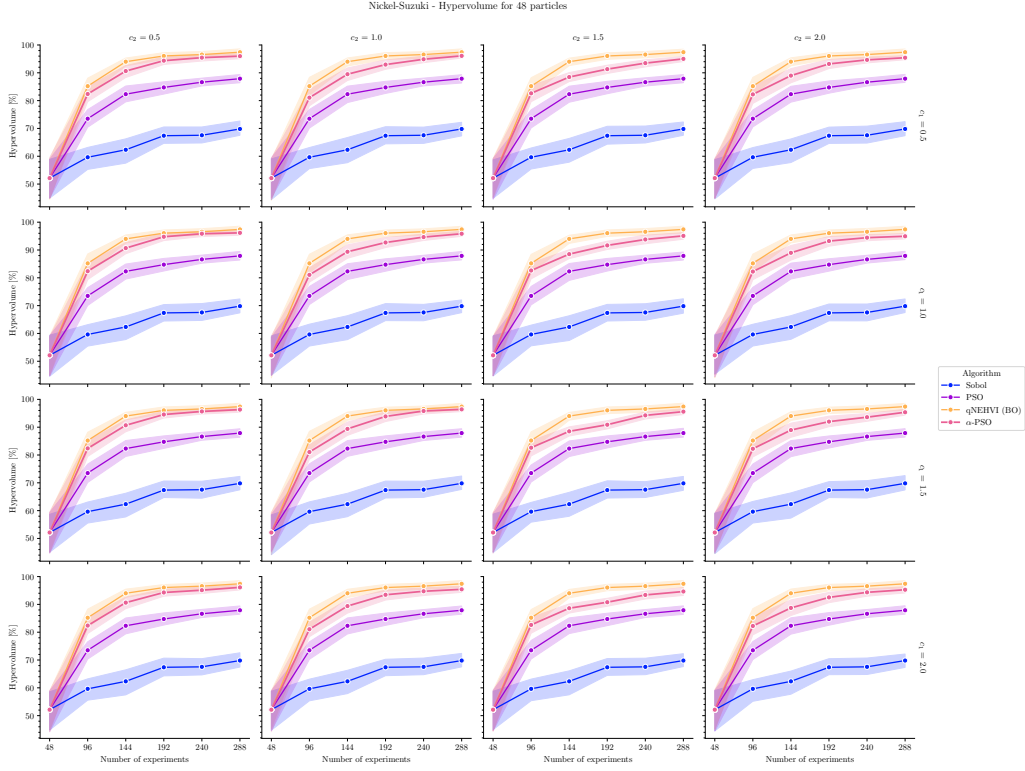

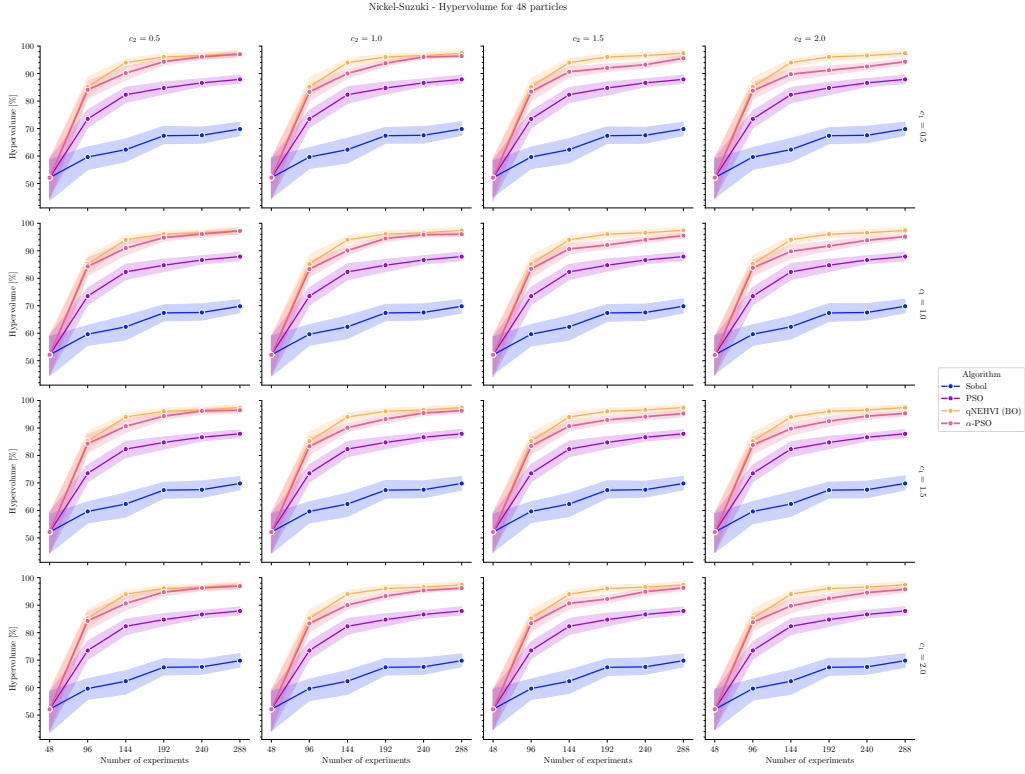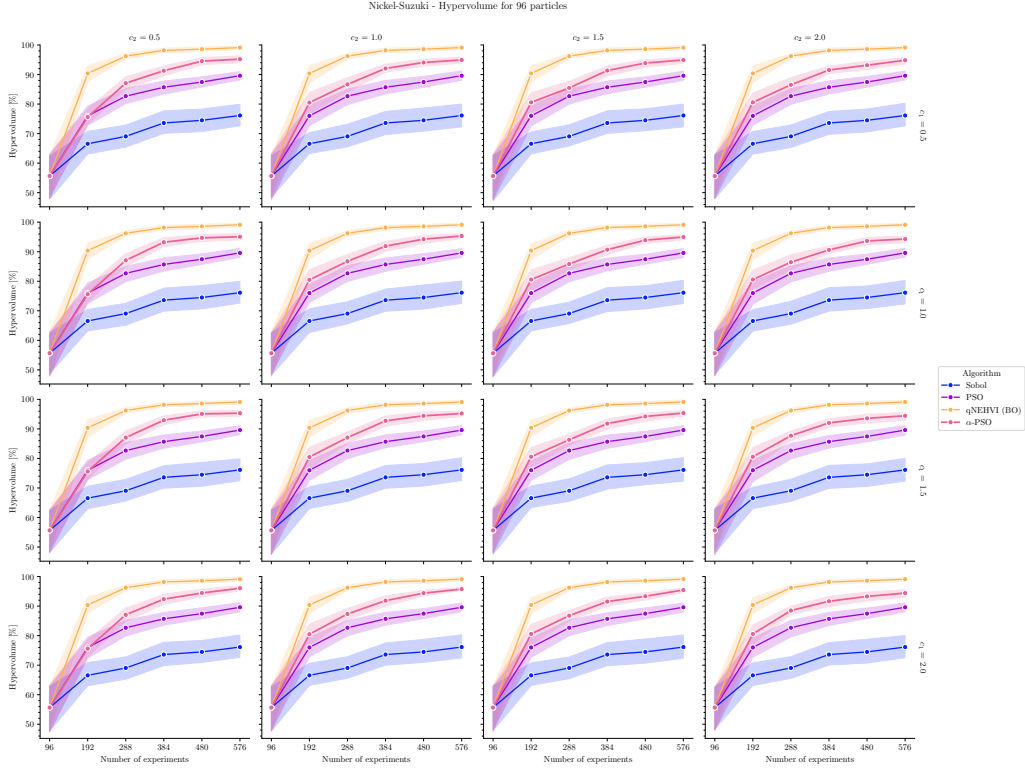

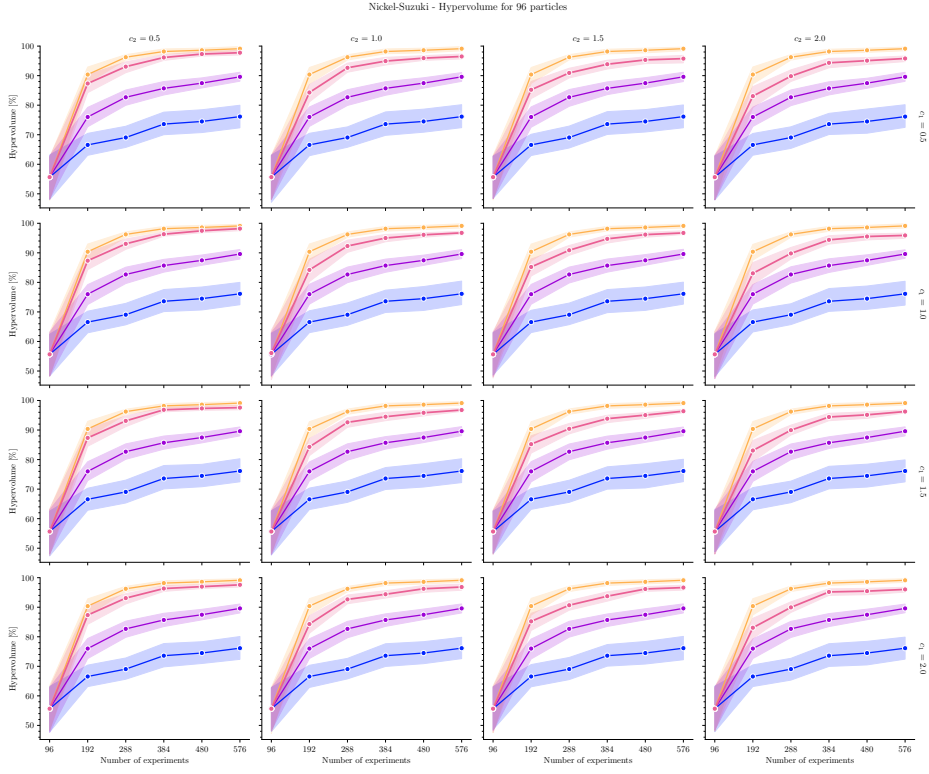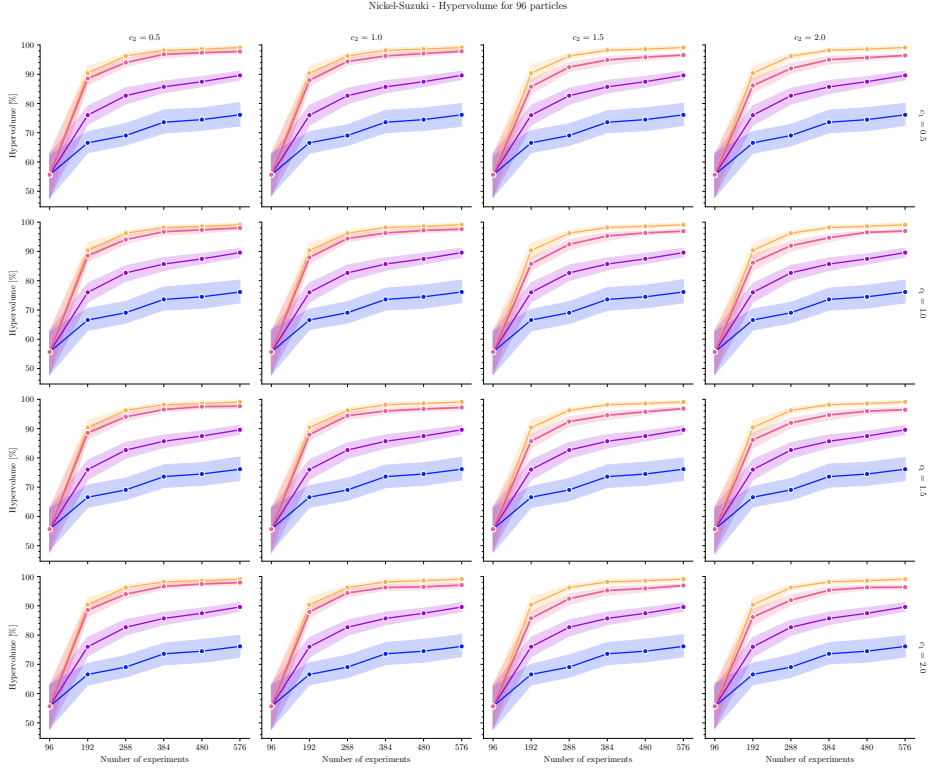

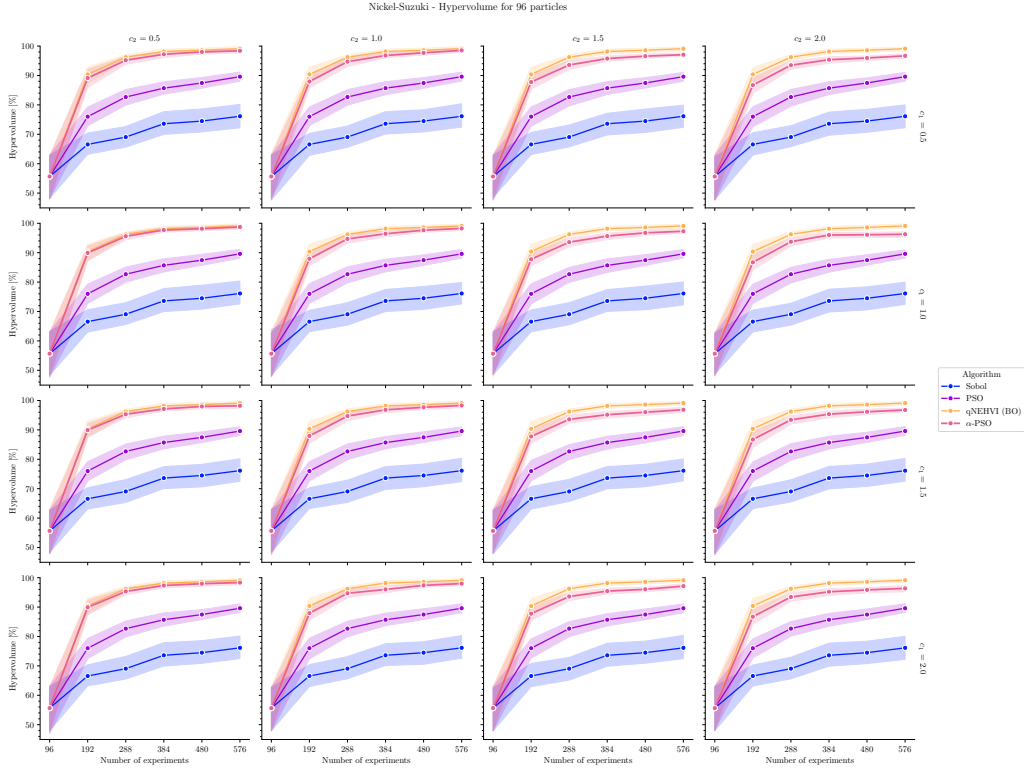

**Supplementary Figure 31:** Ni-Suzuki dataset, batch size 96,  $c_{ml} = 2.0$ .

### 4.3 Effect of particle re-initialisation

We investigated the effect of particle relocation, where the worst-performing particles by reaction outcome are moved directly to the best positions suggested by the acquisition function. We evaluated two strategies: (1) a fixed strategy, where 20% of the worst particles were relocated in each iteration, and (2) an annealed strategy, where the percentage of relocated particles increased from 20% to 50% over the course of the optimisation. For both strategies, we relocated particles after the second iteration to allow the swarm to gather initial information about the landscape.

### 4.3.1 Buchwald-Hartwig dataset

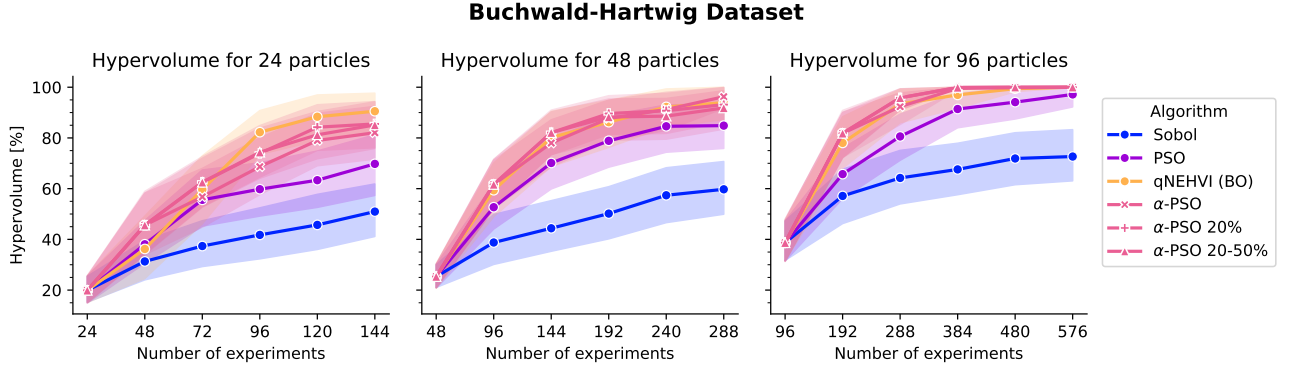

**Supplementary Figure 32:** Buchwald-Hartwig dataset experiments. We compared the hypervolume (%) of the different optimisation algorithms and relocation strategies across 20 random seeds and three batch sizes (24, 48, and 96).  $\alpha$ -PSO used baseline parameters. The shaded regions indicate the 95% confidence interval.

### 4.3.2 Ni-Suzuki dataset

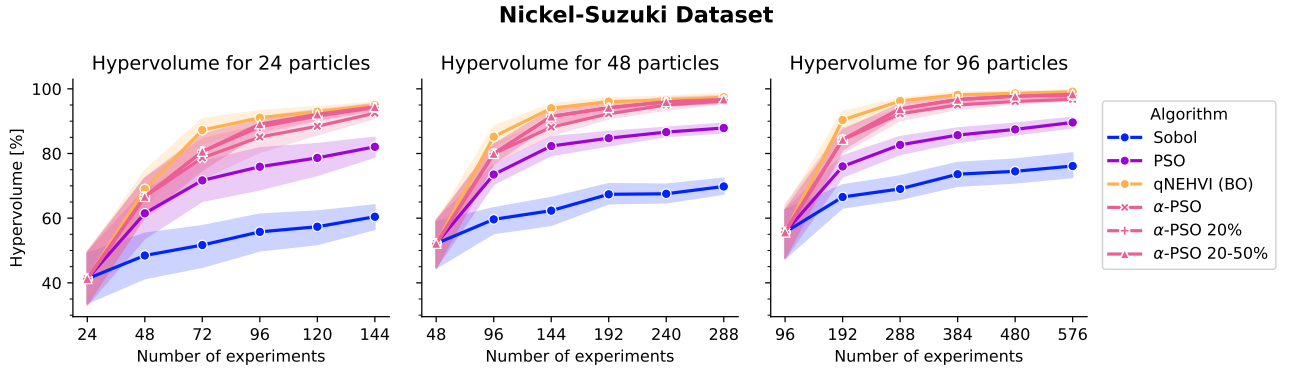

**Supplementary Figure 33:** Ni-Suzuki dataset experiments. We compared the hypervolume (%) of the different optimisation algorithms and relocation strategies across 20 random seeds and three batch sizes (24, 48, and 96).  $\alpha$ -PSO used baseline parameters. The shaded regions indicate the 95% confidence interval.



## 5 Implementation details

All code for model development, computational results, and analyses was implemented in Python 3.12. We used `PyTorch` [28] (v2.4.0), `GPyTorch` [29] (v1.12), and `BoTorch` [30] (v0.11.3) to build our optimisation algorithms, with `PyTorch Lightning` [31] (v2.4.0) employed for reproducible random seed management. `Scikit-learn` [24] (v1.5.1) was utilised for the machine learning pipeline, including data preprocessing, t-SNE visualisation, and k-nearest neighbour calculations. All statistical analyses were conducted using `SciPy` [32] (v1.14.0). `Matplotlib` [33] (v3.9.2) and `seaborn` [34] (v0.13.2) were used for plotting and visualising the results presented in this work. All computations were run on the Roche HPC cluster, using NVIDIA GPUs (A100 Tensor Core GPU, L40S).

## 6 High-throughput experimentation (HTE) platform

We conducted all high-throughput experiments using a parallel experimentation platform custom-designed by UnchainedLabs (Supplementary Figure 34). This system comprises two interconnected Big Kahuna platforms, one of which is further integrated with a LiCONiC LiCotel system. The entire setup is encased within an LC Technology Solutions glove box featuring dual circulation systems, with one dedicated to solid dispensing and another to reaction execution. LCMS analysis was performed using an ACQUITY UPLC I-Class system with QDa from Waters.

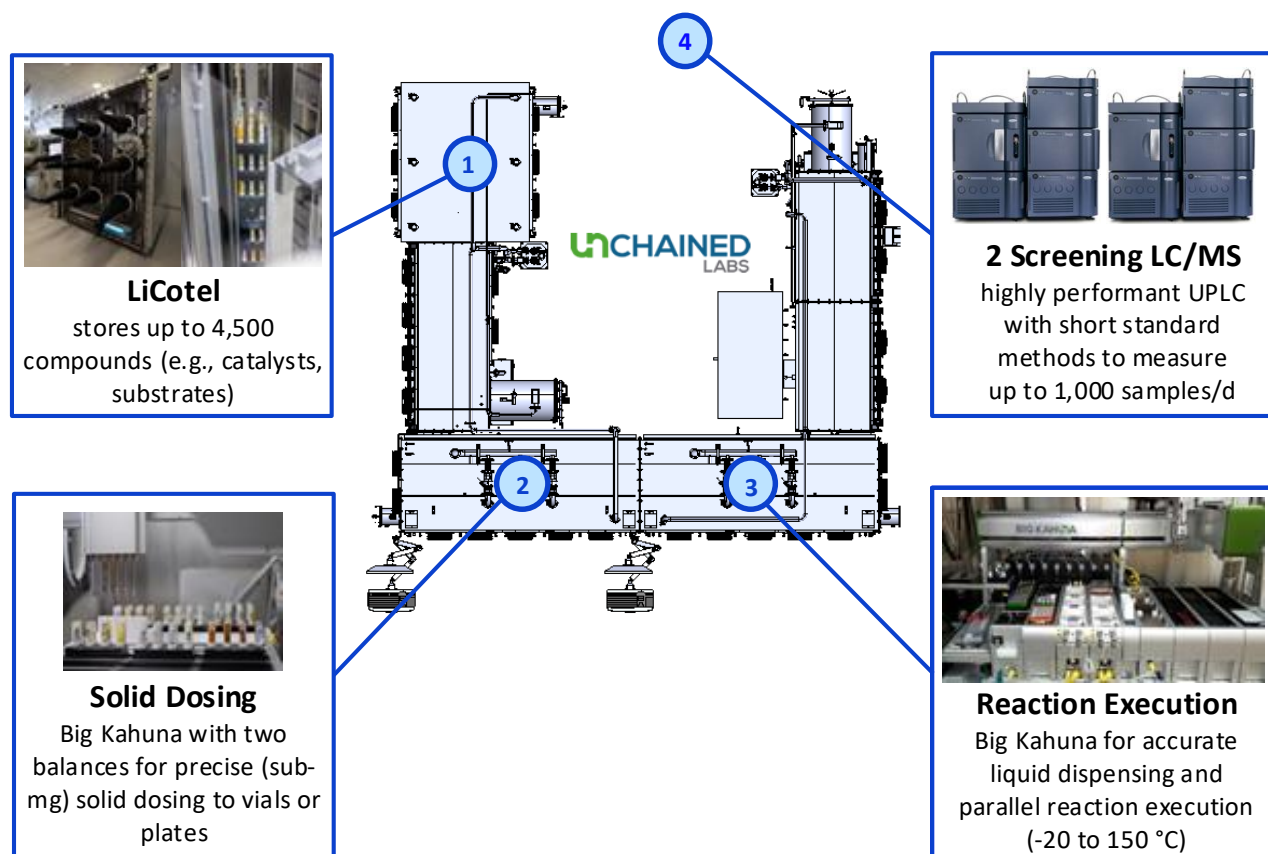

**Supplementary Figure 34:** Schematic overview of the high-throughput experimentation (HTE) set-up.

Solid components were dispensed with a Mettler balance in vial dispense mode, using SV hoppers for precursors, ligands, and substrates, while 10 mL classic hoppers were used for solid additives. For target dispense quantities < 0.4 mg, materials were dispensed as coated ChemBeads (e.g., Pd precursors for the API study). Following automated solid dispensing, liquid components (substrates, liquid additives, and solvents) were manually added using an Eppendorf Multipette E3 single channel pipette (4987000010). Reactions were performed in standard 96-position parallel synthesis reaction blocks (Analytical Sales and Services, SKU: 96960), with V&P Scientific super tumble stir discs (VP 721F-1) for stirring. Data analysis was performed using the HTE OS workflow described by Wuitschik et al. [35] HTE OS is integrated with a SpotFire application that enables tagging of LCMS signals into categories. During analysis, all peaks were tagged accordingly, with peaks corresponding to ligands and precatalyst components designated as “ignore peak”. For LCAP calculations, signals tagged as “solvent” or “ignore peak” were excluded from consideration.

## 7 Prospective application: Sulfonamide coupling

### 7.1 Chemical space description

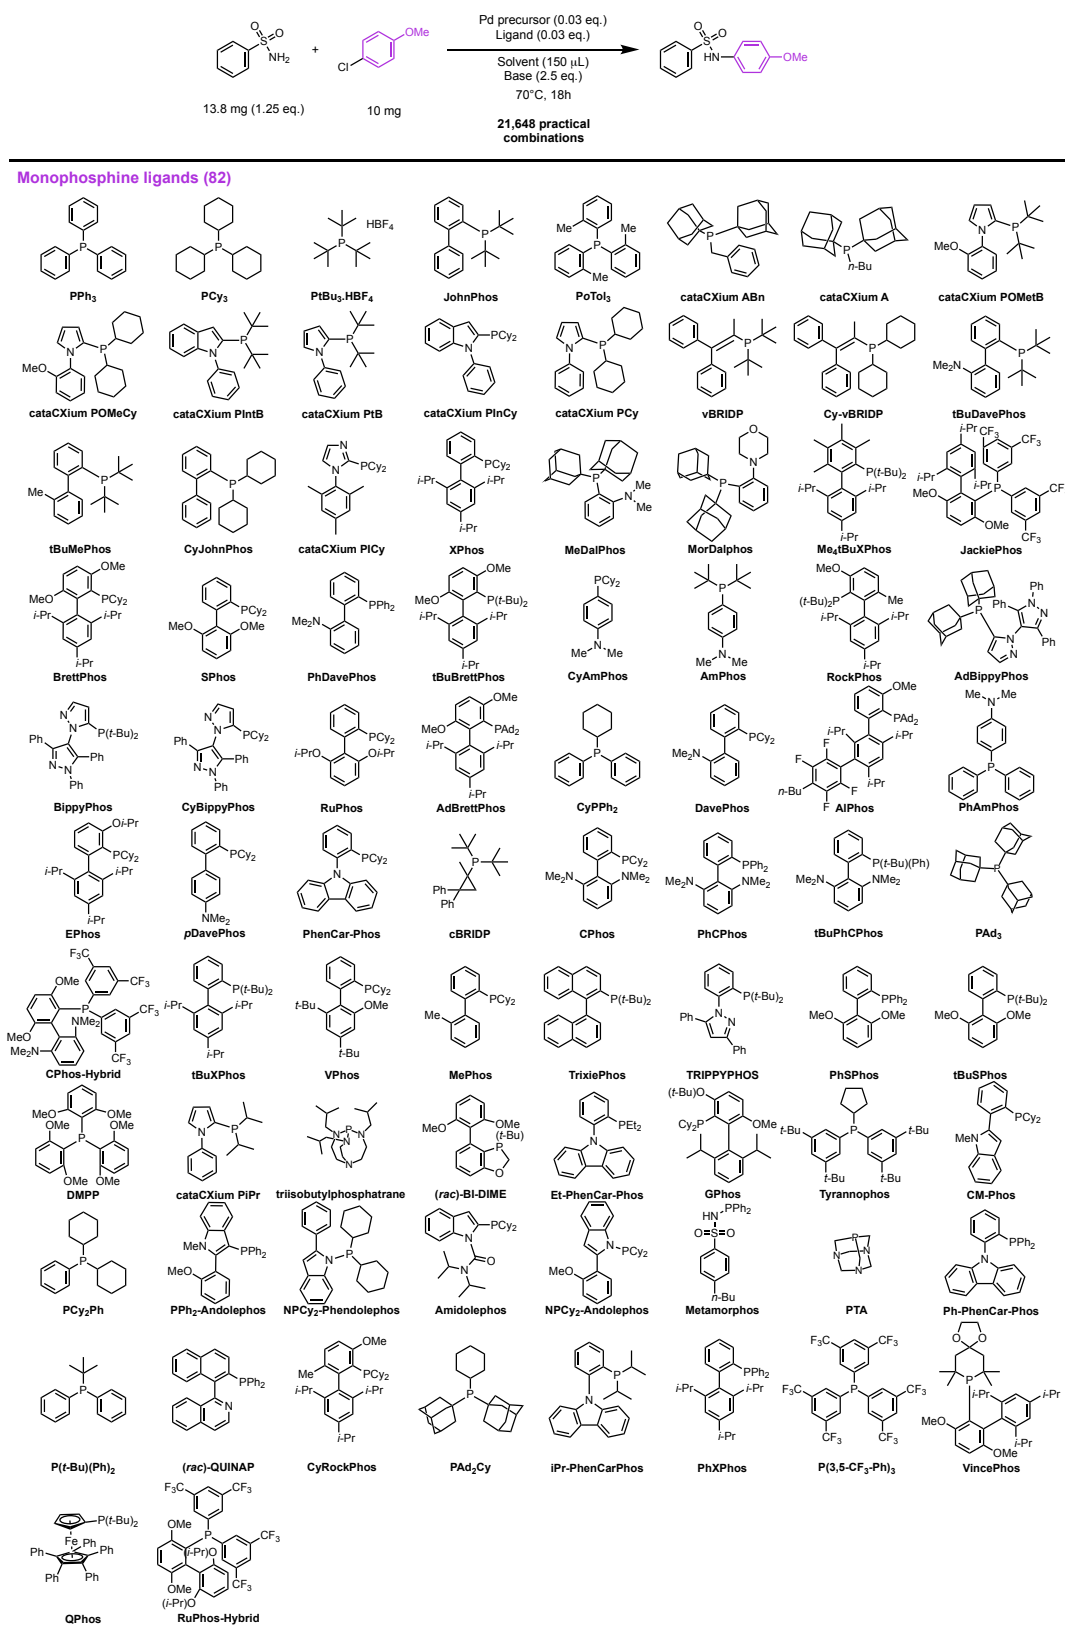

Supplementary Figure 35: Sulfonamide experimental campaign chemical space: 82 ligands.

---

### Solvents (11)

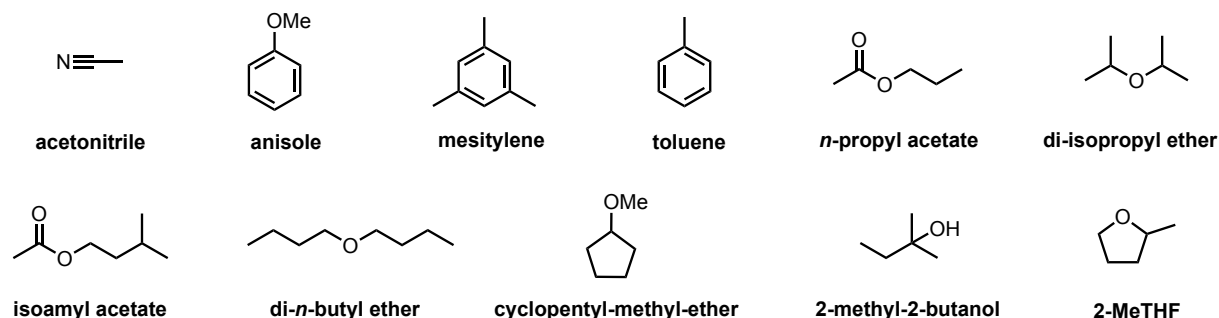

### Bases (8)

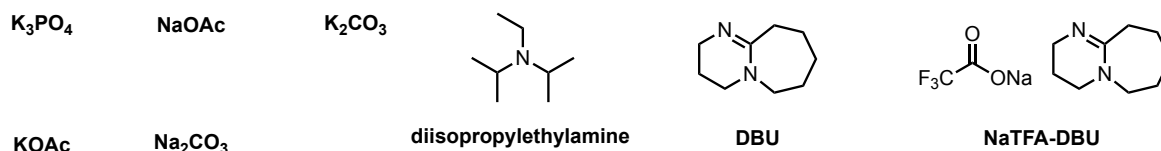

### Precursors (3)

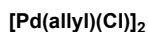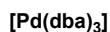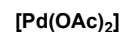

**Supplementary Figure 36:** Sulfonamide experimental campaign chemical space: 11 solvents, 8 bases, and 3 palladium precursors.

## 7.2 HTE experimental procedure

For all HTE plates, the following experimental procedure was performed. Substrates, solid ligands, palladium precursors (on Chembeads) and solid bases were dispensed into 1 mL vials with stirring disks in a 96-well plate. 1-chloro-4-methoxy-benzene, liquid ligands, solvents, and liquid bases were added. The plate was sealed and stirred at 70 °C for 18 h, then cooled to rt. 4/1 MeCN/H<sub>2</sub>O (500  $\mu$ L) was added to each well and shaken for 20 min at rt. 50  $\mu$ L samples were taken and analysed by Liquid Chromatography-Mass Spectroscopy (LC-MS).

## 7.3 Landscape topology analysis

We sampled 96 reaction conditions using Sobol sequences from the defined search space and computed local Lipschitz constants using  $k = 9$  nearest neighbours to assess the reaction landscape roughness of the Pd-catalysed sulfonamide coupling reaction. Landscape topology analysis confirmed our hypothesis from chemical intuition: this sulfonamide coupling exhibited distinctly rough characteristics that closely aligned with our computational Buchwald-Hartwig benchmark ([Supplementary Figure 37](#)). The experimental data showed elevated kurtosis (13.29) values, indicating heavy-tailed distributions with frequent outliers. Notably, the experimental kurtosis (13.29) substantially exceeded the Buchwald-Hartwig benchmark (mean kurtosis: 3.51), suggesting an even rougher reaction landscape, as expected when moving from simulated averages of virtual benchmarks to real experimental data. The Q-Q plot shows that the experimental data points closely followed the upward curvature pattern of the Buchwald-Hartwig benchmark, reaching similar maximum Lipschitz constant ranges

( $\sim 0.095$  compared to  $\sim 0.11$  for the virtual benchmark). The cumulative distribution analysis corroborated these findings between the experimental and virtual Buchwald-Hartwig datasets, with both CDFs showing similar gradual rises and comparable maximum values. Having characterised this case study as a rough reaction landscape, we proceeded with appropriately identified optimisation strategies for such landscapes.

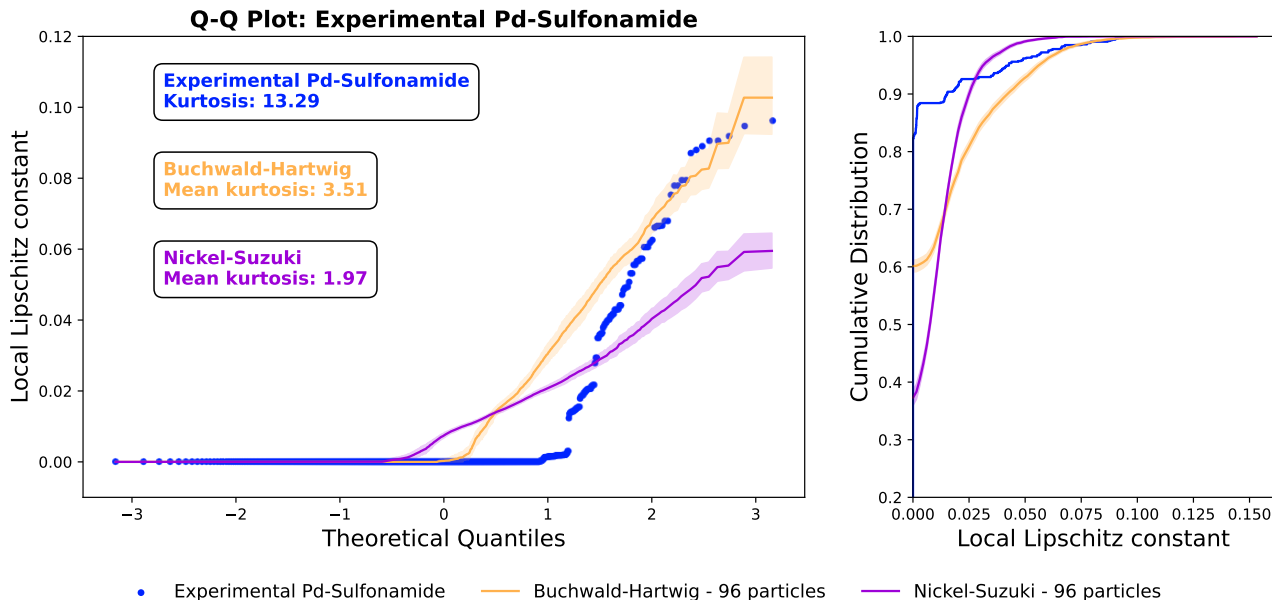

**Supplementary Figure 37: Distribution analysis of the experimental Sulfonamide coupling reaction landscape topology.** Normalised local Lipschitz constants computed from 96 experimental reaction conditions using  $k = 9$  nearest neighbours, compared against virtual benchmark datasets (96-particle Sobol samples averaged across 20 random seeds with confidence bands). (Left) Q-Q plot showing experimental data points plotted against theoretical quantiles from a standard normal distribution, with virtual Buchwald-Hartwig and Ni-Suzuki benchmarks for comparison. (Right) Cumulative distribution functions showing the probability of encountering Lipschitz constants below given thresholds, with experimental data compared to virtual benchmarks. Statistical measures (kurtosis) are displayed for each dataset.

## 7.4 Statistical analysis

To assess the statistical significance of performance differences between methods, we applied the Wilcoxon signed-rank test, a non-parametric test that does not assume normality [36]. This test was performed on the hypervolume values aggregated across all seeds and iterations for a given batch size. We consider three types of alternative hypotheses for Wilcoxon tests: (1) A one-sided test to determine whether the alternative method outperforms the baseline (i.e., has higher hypervolume); (2) A one-sided test to determine whether the alternative method underperforms compared to the baseline; (3) A two-sided test to determine whether there is any statistically significant difference, without assuming directionality. By default, we treat qNEHVI as the baseline for all statistical tests unless stated otherwise.

Null hypothesis  $H_0$  : For  $\mu = 0$ ,  $(X_i, Y_i) \stackrel{d}{=} (Y_i + \mu, X_i - \mu)$

One-side alternative hypothesis  $H_1$  : For  $\mu < 0$ ,  $(X_i, Y_i) \stackrel{d}{=} (Y_i + \mu, X_i - \mu)$

One-side alternative hypothesis  $H_2$  : For  $\mu > 0$ ,  $(X_i, Y_i) \stackrel{d}{=} (Y_i + \mu, X_i - \mu)$

Two-sided alternative hypothesis  $H_3$  : For  $\mu \neq 0$ ,  $(X_i, Y_i) \stackrel{d}{=} (Y_i + \mu, X_i - \mu)$

**Supplementary Table 2:** Statistical comparison of optimisation algorithm performance on the Sulfonamide dataset. Average hypervolume  $\pm$  standard error over 20 random seeds for each iteration, across multiple algorithms.

| Method        | Number of experiments |                  |                  |                  |                  |                  | Wilcoxon signed-rank test |                                 |                       |                                 |                            |                                 |
|---------------|-----------------------|------------------|------------------|------------------|------------------|------------------|---------------------------|---------------------------------|-----------------------|---------------------------------|----------------------------|---------------------------------|
|               | 96                    | 192              | 288              | 384              | 480              | 576              | Method > qNEHVI           |                                 | qNEHVI > Method       |                                 | Method $\neq$ qNEHVI       |                                 |
|               |                       |                  |                  |                  |                  |                  | p-value<br>med(D) > 0     | Significance<br>$\alpha = 0.05$ | p-value<br>med(D) < 0 | Significance<br>$\alpha = 0.05$ | p-value<br>med(D) $\neq 0$ | Significance<br>$\alpha = 0.05$ |
| Sobol         | 36.01 $\pm$ 4.74      | 50.5 $\pm$ 5.5   | 60.24 $\pm$ 5.31 | 74.66 $\pm$ 4.94 | 77.48 $\pm$ 4.68 | 79.49 $\pm$ 4.63 | 1.0                       | ✗                               | 0.0                   | ✓                               | 0.0                        | ✓                               |
| PSO           | 36.01 $\pm$ 4.74      | 71.85 $\pm$ 5.48 | 85.26 $\pm$ 5.08 | 95.12 $\pm$ 2.31 | 98.1 $\pm$ 0.74  | 99.28 $\pm$ 0.25 | 0.4027                    | ✗                               | 0.5973                | ✗                               | 0.8054                     | ✗                               |
| qNEHVI (BO)   | 36.01 $\pm$ 4.74      | 65.49 $\pm$ 4.68 | 87.48 $\pm$ 3.87 | 95.49 $\pm$ 1.92 | 97.42 $\pm$ 1.69 | 98.66 $\pm$ 1.22 | -                         | -                               | -                     | -                               | -                          | -                               |
| $\alpha$ -PSO | 36.01 $\pm$ 4.74      | 74.51 $\pm$ 3.88 | 95.44 $\pm$ 1.38 | 99.17 $\pm$ 0.72 | 100.0 $\pm$ 0.0  | 100.0 $\pm$ 0.0  | 0.0                       | ✓                               | 1.0                   | ✗                               | 0.0001                     | ✓                               |

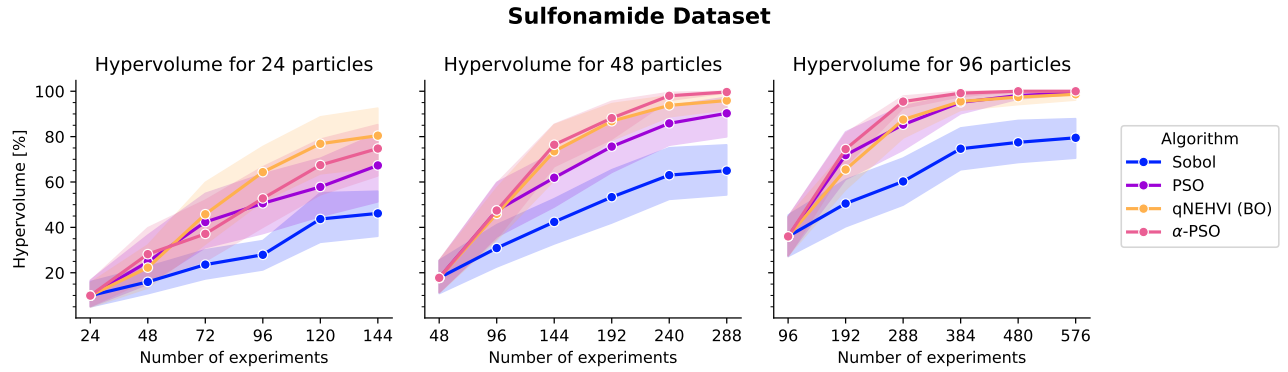

**Supplementary Figure 38:** Performance of different optimisation algorithms on the Sulfonamide dataset over 20 random seeds and three batch sizes (24, 48, and 96). The shaded regions indicate the 95% confidence interval.

## 8 Prospective application: Suzuki-Miyaura reaction

### 8.1 Chemical space description

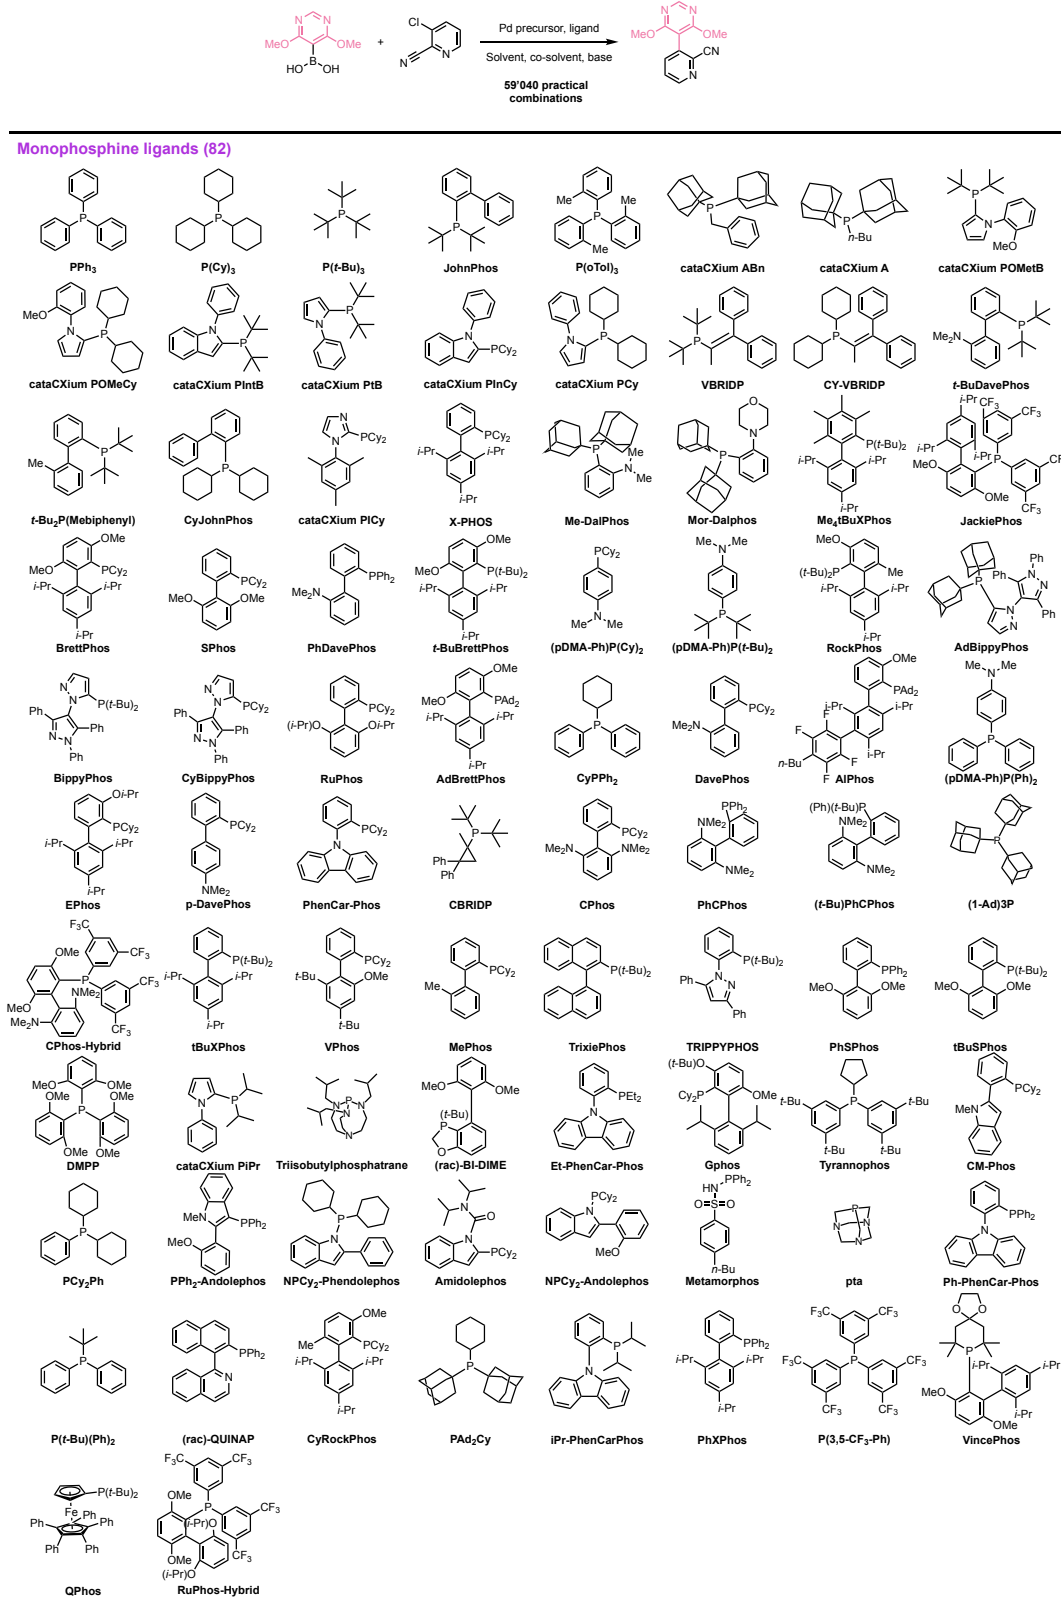

Supplementary Figure 39: Suzuki-Miyaura reaction experimental campaign chemical space: 82 ligands.

---

### Solvents (12)

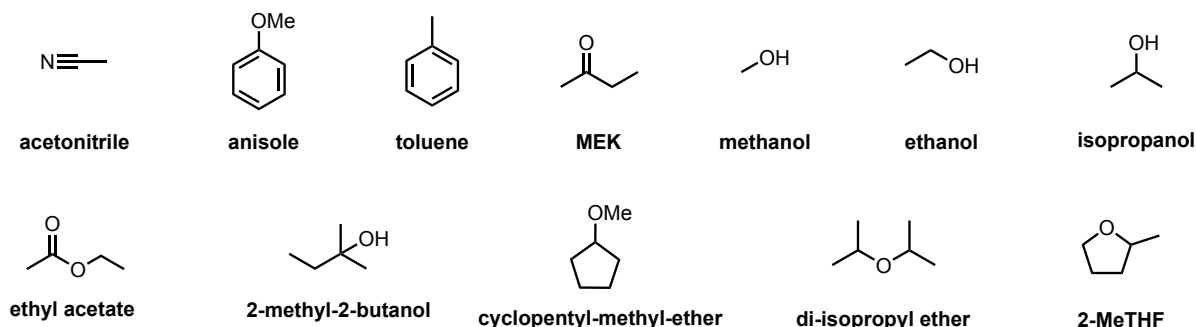

---

### Bases (10)

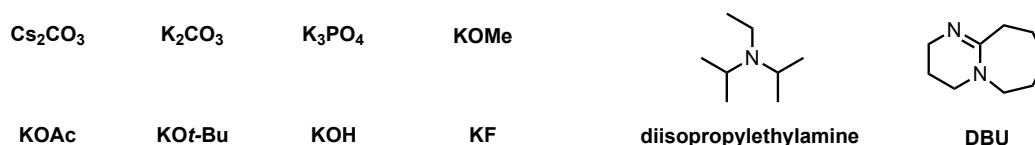

---

### Precursors (3)

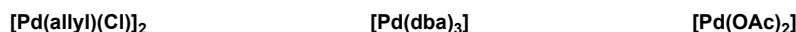

---

### Co-solvents (2)

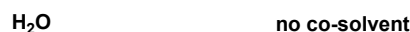

**Supplementary Figure 40:** Suzuki-Miyaura reaction experimental campaign chemical space: 12 solvents, 2 co-solvents, 10 bases, and 3 palladium precursors.

## 8.2 HTE experimental procedure

For all HTE plates, the following experimental procedure was performed. Substrates, solid ligands, palladium precursors (on Chembeads) and solid bases were dispensed into 1 mL vials with stirring disks in a 96-well plate. Liquid ligands, solvents, co-solvents, and liquid bases were added. The plate was sealed and stirred at 70 °C for 20 h, then cooled to rt. 4/1 MeCN/H<sub>2</sub>O (500 μL) was added to each well and shaken for 20 min at rt. 50 μL samples were taken and analysed by Liquid Chromatography-Mass Spectroscopy (LC-MS).

## 8.3 Landscape topology analysis

We sampled 96 reaction conditions using Sobol sequences from the defined search space and computed local Lipschitz constants using  $k = 9$  nearest neighbours to assess the reaction landscape roughness of the Pd-catalysed Suzuki coupling reaction. Landscape topology analysis showed that this Suzuki coupling exhibited distinctly smooth characteristics that closely aligned with our computational Ni-Suzuki benchmark (Supplementary figure 41). The experimental data showed moderately low kurtosis (1.93) values, indicating relatively condensed distributions with minimal extreme outliers, characteristic of smooth reaction spaces with few reactivity cliffs. The Q-Q plot revealed that experimental



data points followed a gentle upward curve that closely tracked the Ni-Suzuki benchmark pattern, with maximum Lipschitz constants reaching similar moderate ranges ( $\sim 0.07$  compared to  $\sim 0.06$  for the virtual benchmark). While these values are slightly elevated compared to the virtual Ni-Suzuki benchmark, this is an expected overestimation when comparing single experimental realisations to averaged virtual benchmarks across multiple seeds. The cumulative distribution analysis corroborated these findings, with the experimental CDF showing a steep initial rise similar to the Ni-Suzuki profile, confirming the predominance of low-Lipschitz regions where reaction conditions produce proportional and predictable changes in outcomes. Having characterised this as a smooth reaction landscape, we proceeded with optimisation parameters specifically tuned for such chemical spaces.

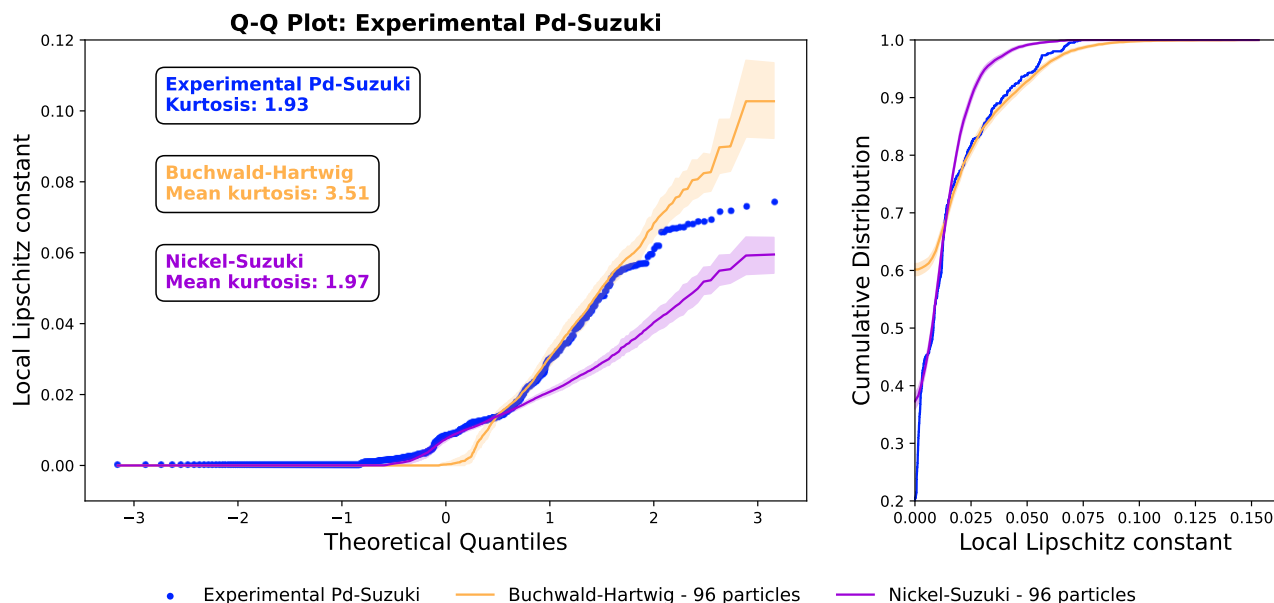

**Supplementary Figure 41: Distribution analysis of the experimental Suzuki coupling reaction landscape topology.** Normalised local Lipschitz constants computed from 96 experimental reaction conditions using  $k = 9$  nearest neighbours, compared against virtual benchmark datasets (96-particle Sobol samples averaged across 20 random seeds with confidence bands). (Left) Q-Q plot showing experimental data points plotted against theoretical quantiles from a standard normal distribution, with virtual Buchwald-Hartwig and Ni-Suzuki benchmarks for comparison. (Right) Cumulative distribution functions showing the probability of encountering Lipschitz constants below given thresholds, with experimental data compared to virtual benchmarks. Statistical measures (kurtosis) are displayed for each dataset.

## References

- [1] A. P. Guerreiro, C. M. Fonseca, L. Paquete, *ACM Computing Surveys* **2022**, *54*, 1–42, DOI [10.1145/3453474](https://doi.org/10.1145/3453474).
- [2] S. Daulton, M. Balandat, E. Bakshy in *Advances in Neural Information Processing Systems, Vol. 33*, Curran Associates, Inc., **2020**, pp. 9851–9864.
- [3] S. Daulton, M. Balandat, E. Bakshy, Parallel Bayesian Optimization of Multiple Noisy Objectives with Expected Hypervolume Improvement, **2021**, DOI [10.48550/arXiv.2105.08195](https://doi.org/10.48550/arXiv.2105.08195), <http://arxiv.org/abs/2105.08195> (visited on 11/12/2024), pre-published.
- [4] J. J. Dotson, L. van Dijk, J. C. Timmerman, S. Grosslight, R. C. Walroth, F. Gosselin, K. Püntener, K. A. Mack, M. S. Sigman, *Journal of the American Chemical Society* **2023**, *145*, 110–121, DOI [10.1021/jacs.2c08513](https://doi.org/10.1021/jacs.2c08513).
- [5] J. W. Sin, S. L. Chau, R. P. Burwood, K. Püntener, R. Bigler, P. Schwaller, *Nature Communications* **2025**, *16*, 6464, DOI [10.1038/s41467-025-61803-0](https://doi.org/10.1038/s41467-025-61803-0).
- [6] J. A. G. Torres, S. H. Lau, P. Anchuri, J. M. Stevens, J. E. Tabora, J. Li, A. Borovika, R. P. Adams, A. G. Doyle, *Journal of the American Chemical Society* **2022**, *144*, 19999–20007, DOI [10.1021/jacs.2c08592](https://doi.org/10.1021/jacs.2c08592).
- [7] D. M. Dalton, R. C. Walroth, C. Rouget-Virbel, K. A. Mack, F. D. Toste, *Journal of the American Chemical Society* **2024**, *146*, 15779–15786, DOI [10.1021/jacs.4c01616](https://doi.org/10.1021/jacs.4c01616).
- [8] T. Gensch, G. dos Passos Gomes, P. Friederich, E. Peters, T. Gaudin, R. Pollice, K. Jorner, A. Nigam, M. Lindner-D’Addario, M. S. Sigman, A. Aspuru-Guzik, *Journal of the American Chemical Society* **2022**, *144*, 1205–1217, DOI [10.1021/jacs.1c09718](https://doi.org/10.1021/jacs.1c09718).
- [9] L. Moity, M. Durand, A. Benazzouz, C. Pierlot, V. Molinier, J.-M. Aubry, *Green Chemistry* **2012**, *14*, 1132–1145, DOI [10.1039/C2GC16515E](https://doi.org/10.1039/C2GC16515E).
- [10] P. I. Frazier, A Tutorial on Bayesian Optimization, **2018**, DOI [10.48550/arXiv.1807.02811](https://doi.org/10.48550/arXiv.1807.02811), <http://arxiv.org/abs/1807.02811> (visited on 08/12/2025), pre-published.
- [11] B. J. Shields, J. Stevens, J. Li, M. Parasram, F. Damani, J. I. M. Alvarado, J. M. Janey, R. P. Adams, A. G. Doyle, *Nature* **2021**, *590*, 89–96, DOI [10.1038/s41586-021-03213-y](https://doi.org/10.1038/s41586-021-03213-y).
- [12] C. J. Taylor, A. Pomberger, K. C. Felton, R. Grainger, M. Barecka, T. W. Chamberlain, R. A. Bourne, C. N. Johnson, A. A. Lapkin, *Chemical Reviews* **2023**, *123*, 3089–3126, DOI [10.1021/acs.chemrev.2c00798](https://doi.org/10.1021/acs.chemrev.2c00798).
- [13] B. Mahjour, R. Zhang, Y. Shen, A. McGrath, R. Zhao, O. G. Mohamed, Y. Lin, Z. Zhang, J. L. Douthwaite, A. Tripathi, T. Cernak, *Nature Communications* **2023**, *14*, 3924, DOI [10.1038/s41467-023-39531-0](https://doi.org/10.1038/s41467-023-39531-0).
- [14] A. Buitrago Santanilla, E. L. Regalado, T. Pereira, M. Shevlin, K. Bateman, L.-C. Campeau, J. Schneeweis, S. Berritt, Z.-C. Shi, P. Nantermet, Y. Liu, R. Helmy, C. J. Welch, P. Vachal, I. W. Davies, T. Cernak, S. D. Dreher, *Science* **2015**, *347*, 49–53, DOI [10.1126/science.1259203](https://doi.org/10.1126/science.1259203).
- [15] W. H. Bangyal, K. Nisar, A. A. B. Ag. Ibrahim, M. R. Haque, J. J. P. C. Rodrigues, D. B. Rawat, *Applied Sciences* **2021**, *11*, 7591, DOI [10.3390/app11167591](https://doi.org/10.3390/app11167591).
- [16] J. Kennedy, R. Eberhart in *Proceedings of ICNN’95 - International Conference on Neural Networks, Vol. 4*, ICNN’95 - International Conference on Neural Networks, IEEE, Perth, WA, Australia, **1995**, pp. 1942–1948, DOI [10.1109/ICNN.1995.488968](https://doi.org/10.1109/ICNN.1995.488968).
- [17] T. Blackwell, J. Kennedy, *IEEE Transactions on Evolutionary Computation* **2019**, *23*, 689–702, DOI [10.1109/TEVC.2018.2880894](https://doi.org/10.1109/TEVC.2018.2880894).

- [18] A. McNabb, M. Gardner, K. Seppi in 2009 IEEE Congress on Evolutionary Computation, 2009 IEEE Congress on Evolutionary Computation (CEC), IEEE, Trondheim, Norway, **2009**, pp. 712–719, DOI [10.1109/CEC.2009.4983015](https://doi.org/10.1109/CEC.2009.4983015).
- [19] In Proceedings of the International Joint Conference on Computational Intelligence, International Conference on Evolutionary Computation, SciTePress - Science and Technology Publications, Funchal - Madeira, Portugal, **2009**, pp. 152–159, DOI [10.5220/0002324801520159](https://doi.org/10.5220/0002324801520159).
- [20] B.-I. Koh, A. D. George, R. T. Haftka, B. J. Fregly, *International Journal for Numerical Methods in Engineering* **2006**, *67*, 578–595, DOI [10.1002/nme.1646](https://doi.org/10.1002/nme.1646).
- [21] J. Jakubik, A. Binding, S. Feuerriegel, *European Journal of Operational Research* **2021**, *295*, 157–169, DOI [10.1016/j.ejor.2021.02.053](https://doi.org/10.1016/j.ejor.2021.02.053).
- [22] F. Häse, M. Aldeghi, R. J. Hickman, L. M. Roch, M. Christensen, E. Liles, J. E. Hein, A. Aspuru-Guzik, *Machine Learning: Science and Technology* **2021**, *2*, 035021, DOI [10.1088/2632-2153/abedc8](https://doi.org/10.1088/2632-2153/abedc8).
- [23] K. C. Felton, J. G. Rittig, A. A. Lapkin, *Chemistry-Methods* **2021**, *1*, 116–122, DOI [10.1002/cmtd.202000051](https://doi.org/10.1002/cmtd.202000051).
- [24] F. Pedregosa, G. Varoquaux, A. Gramfort, V. Michel, B. Thirion, O. Grisel, M. Blondel, P. Prettenhofer, R. Weiss, V. Dubourg, J. Vanderplas, A. Passos, D. Cournapeau, M. Brucher, M. Perrot, É. Duchesnay, *J. Mach. Learn. Res.* **2011**, *12*, 2825–2830.
- [25] M. Jordan, A. G. Dimakis in *Advances in Neural Information Processing Systems, Vol. 33*, Curran Associates, Inc., **2020**, pp. 7344–7353.
- [26] K. Taunk, S. De, S. Verma, A. Swetapadma in 2019 International Conference on Intelligent Computing and Control Systems (ICCS), 2019 International Conference on Intelligent Computing and Control Systems (ICCS), **2019**, pp. 1255–1260, DOI [10.1109/ICCS45141.2019.9065747](https://doi.org/10.1109/ICCS45141.2019.9065747).
- [27] J. Zhang, N. Sugisawa, K. C. Felton, S. Fuse, A. A. Lapkin, *Reaction Chemistry & Engineering* **2024**, *9*, 706–712, DOI [10.1039/D3RE00502J](https://doi.org/10.1039/D3RE00502J).
- [28] A. Paszke, S. Gross, F. Massa, A. Lerer, J. Bradbury, G. Chanan, T. Killeen, Z. Lin, N. Gimeshain, L. Antiga, A. Desmaison, A. Köpf, E. Yang, Z. DeVito, M. Raison, A. Tejani, S. Chilamkurthy, B. Steiner, L. Fang, J. Bai, S. Chintala in *Proceedings of the 33rd International Conference on Neural Information Processing Systems*, 721, Curran Associates Inc., Red Hook, NY, USA, **2019**, pp. 8026–8037.
- [29] J. R. Gardner, G. Pleiss, D. Bindel, K. Q. Weinberger, A. G. Wilson in *Proceedings of the 32nd International Conference on Neural Information Processing Systems*, Curran Associates Inc., Red Hook, NY, USA, **2018**, pp. 7587–7597.
- [30] M. Balandat, B. Karrer, D. Jiang, S. Daulton, B. Letham, A. G. Wilson, E. Bakshy in *Advances in Neural Information Processing Systems, Vol. 33*, Curran Associates, Inc., **2020**, pp. 21524–21538.
- [31] W. Falcon, J. Borovec, A. Wälchli, N. Eggert, J. Schock, J. Jordan, N. Skafte, Ir1dXD, V. Bereznyuk, E. Harris, T. Murrell, P. Yu, S. Præsius, T. Addair, J. Zhong, D. Lipin, S. Uchida, S. Bapat, H. Schröter, B. Dayma, A. Karnachev, A. Kulkarni, S. Komatsu, Martin.B, J.-B. SCHIRATTI, H. Mary, D. Byrne, C. Eyzaguirre, cinjon, A. Bakhtin, *PyTorchLightning/Pytorch-Lightning: 0.7.6 Release*, Zenodo, **2020**, DOI [10.5281/zenodo.3828935](https://doi.org/10.5281/zenodo.3828935).

- [32] P. Virtanen, R. Gommers, T. E. Oliphant, M. Haberland, T. Reddy, D. Cournapeau, E. Burovski, P. Peterson, W. Weckesser, J. Bright, S. J. van der Walt, M. Brett, J. Wilson, K. J. Millman, N. Mayorov, A. R. J. Nelson, E. Jones, R. Kern, E. Larson, C. J. Carey, Í. Polat, Y. Feng, E. W. Moore, J. VanderPlas, D. Laxalde, J. Perktold, R. Cimrman, I. Henriksen, E. A. Quintero, C. R. Harris, A. M. Archibald, A. H. Ribeiro, F. Pedregosa, P. van Mulbregt, *Nature Methods* **2020**, *17*, 261–272, DOI [10.1038/s41592-019-0686-2](https://doi.org/10.1038/s41592-019-0686-2).
- [33] J. D. Hunter, *Computing in Science & Engineering* **2007**, *9*, 90–95, DOI [10.1109/MCSE.2007.55](https://doi.org/10.1109/MCSE.2007.55).
- [34] M. L. Waskom, *Journal of Open Source Software* **2021**, *6*, 3021, DOI [10.21105/joss.03021](https://doi.org/10.21105/joss.03021).
- [35] G. Wuitschik, V. Jost, T. Schindler, M. Jakubik, *Organic Process Research & Development* **2024**, *28*, 2875–2884, DOI [10.1021/acs.oprd.4c00160](https://doi.org/10.1021/acs.oprd.4c00160).
- [36] J. W. Pratt, *Journal of the American Statistical Association* **1959**, *54*, 655–667, DOI [10.1080/01621459.1959.10501526](https://doi.org/10.1080/01621459.1959.10501526).
